# Supplementary material for: Enabling Roll-up and Drill-down Operations in News Exploration with Knowledge Graphs for Due Diligence and Risk Management
Source: arXiv:2405.04929 source file (2024-05-08)
Supplement: Supplementary file 1 [file appendix-interface.tex]

\begin{figure*}[ht]
\centering
\subfloat[search by concepts]
  {\includegraphics[width=.85\linewidth]{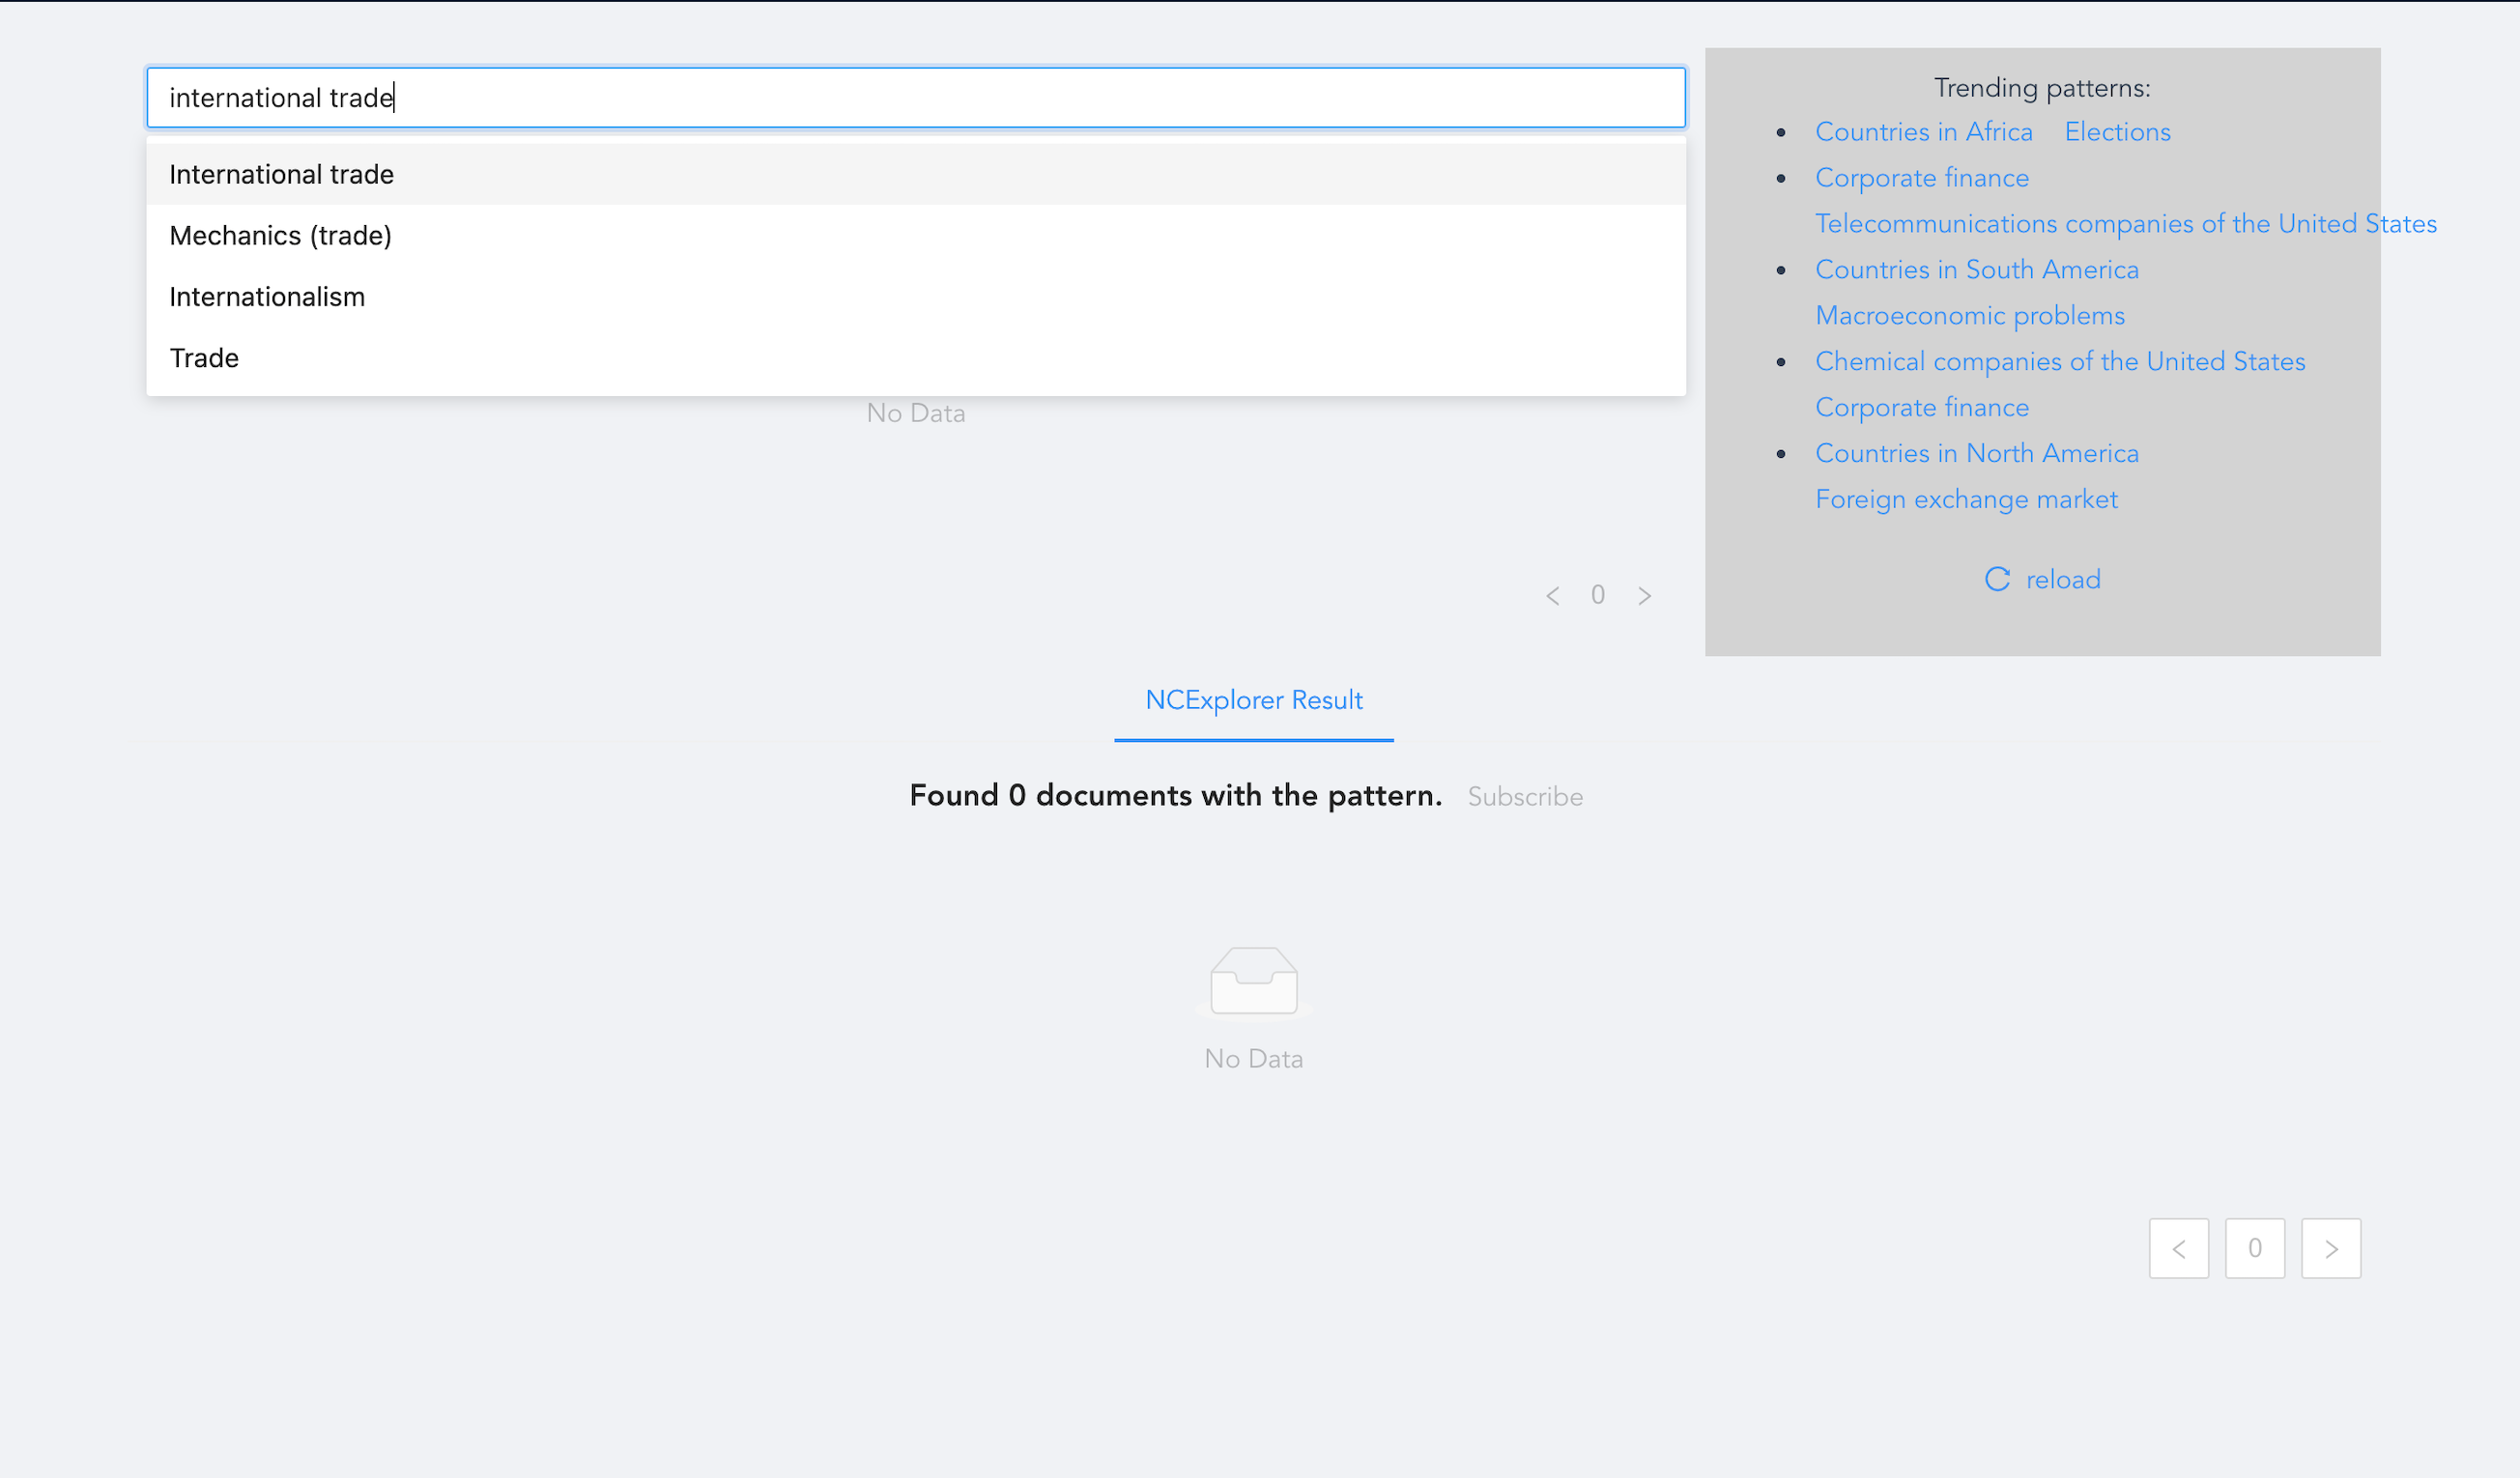}}\hfill
\subfloat[search result]
  {\includegraphics[width=.85\linewidth]{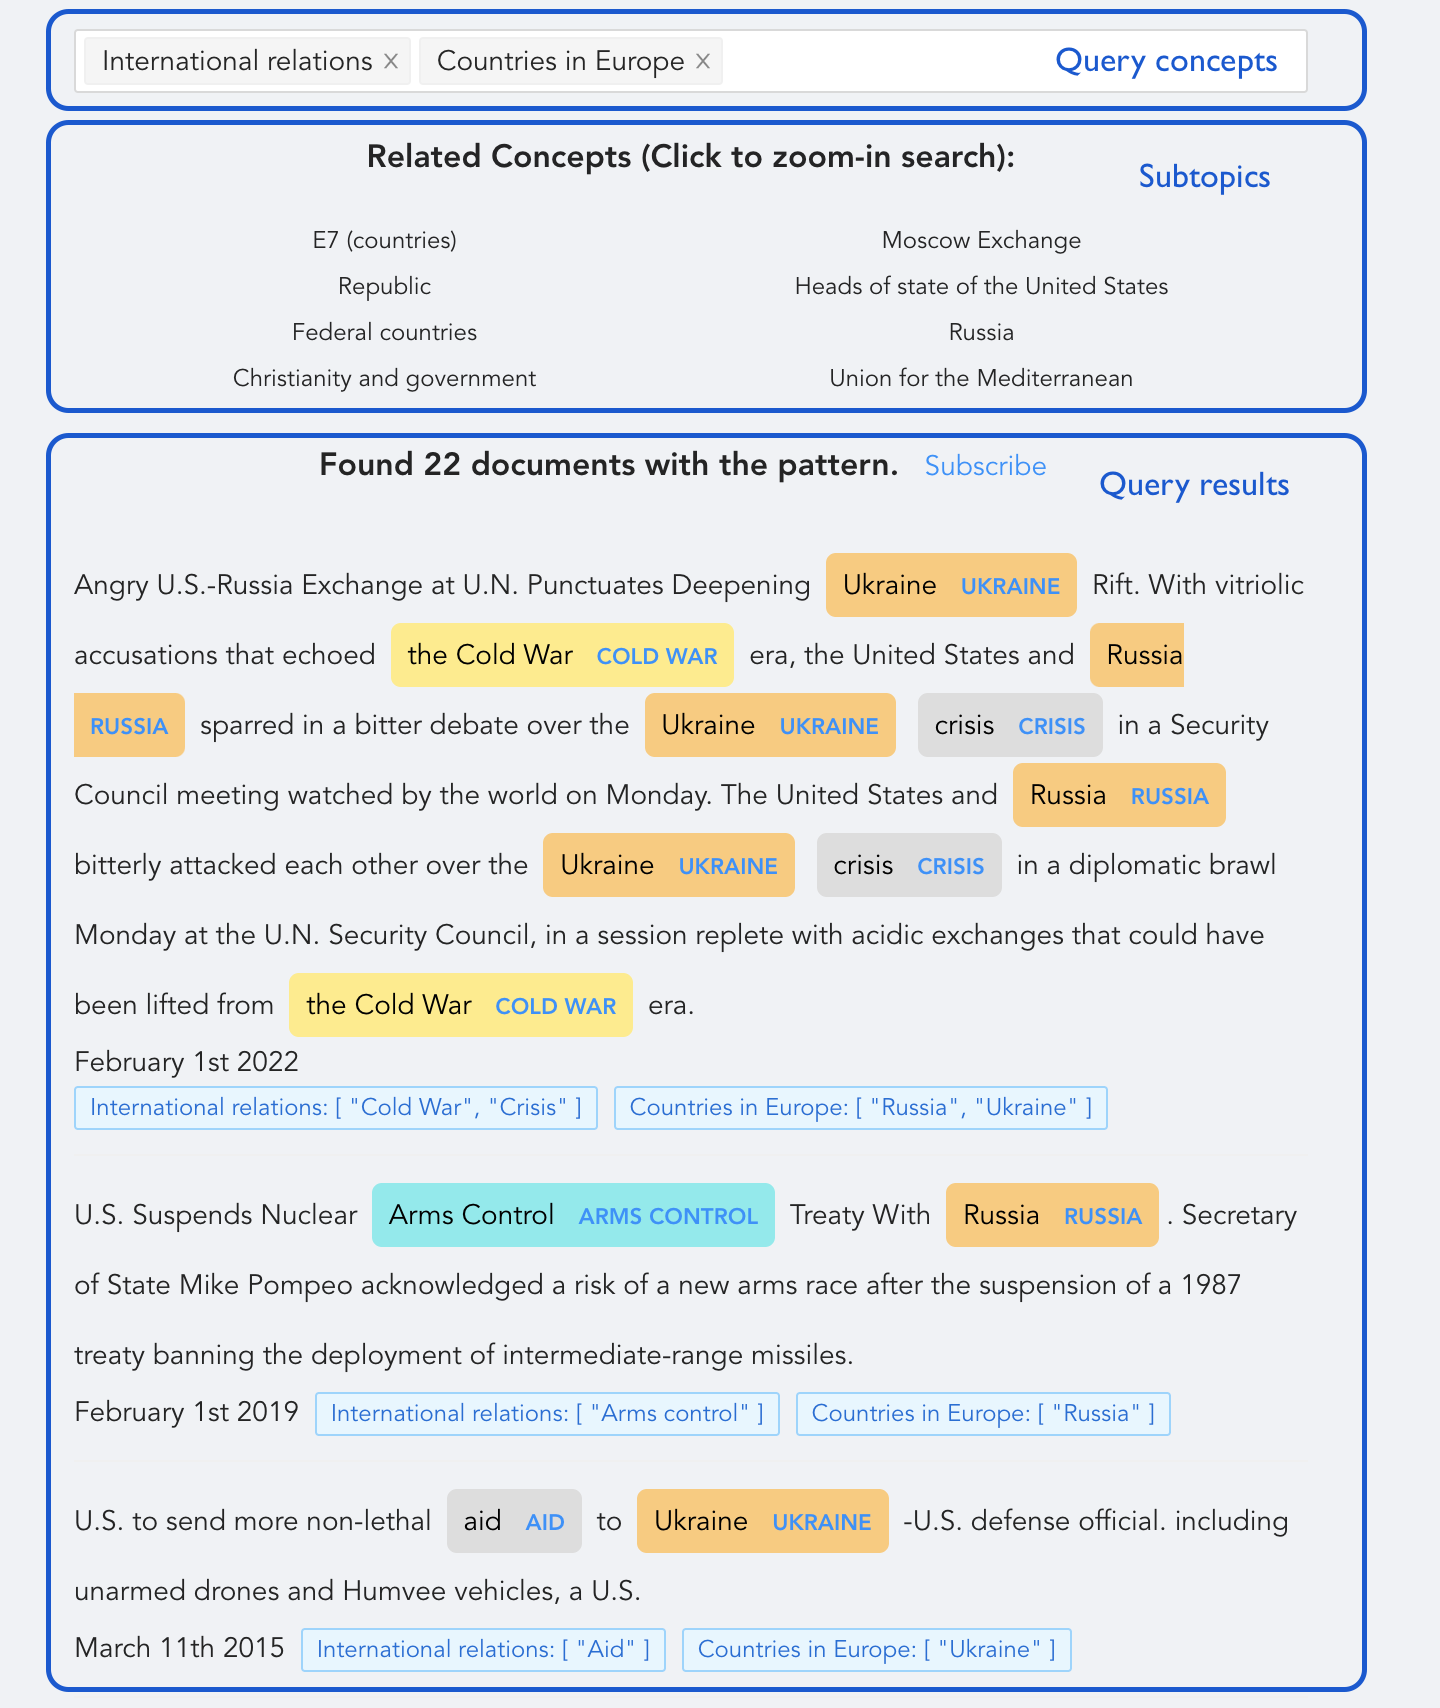}}\hfill
  \caption{}
 \end{figure*}%
 
\begin{figure*}[ht]\ContinuedFloat
\centering
\subfloat[select subtopics via instance entities]
  {\includegraphics[width=.85\linewidth]{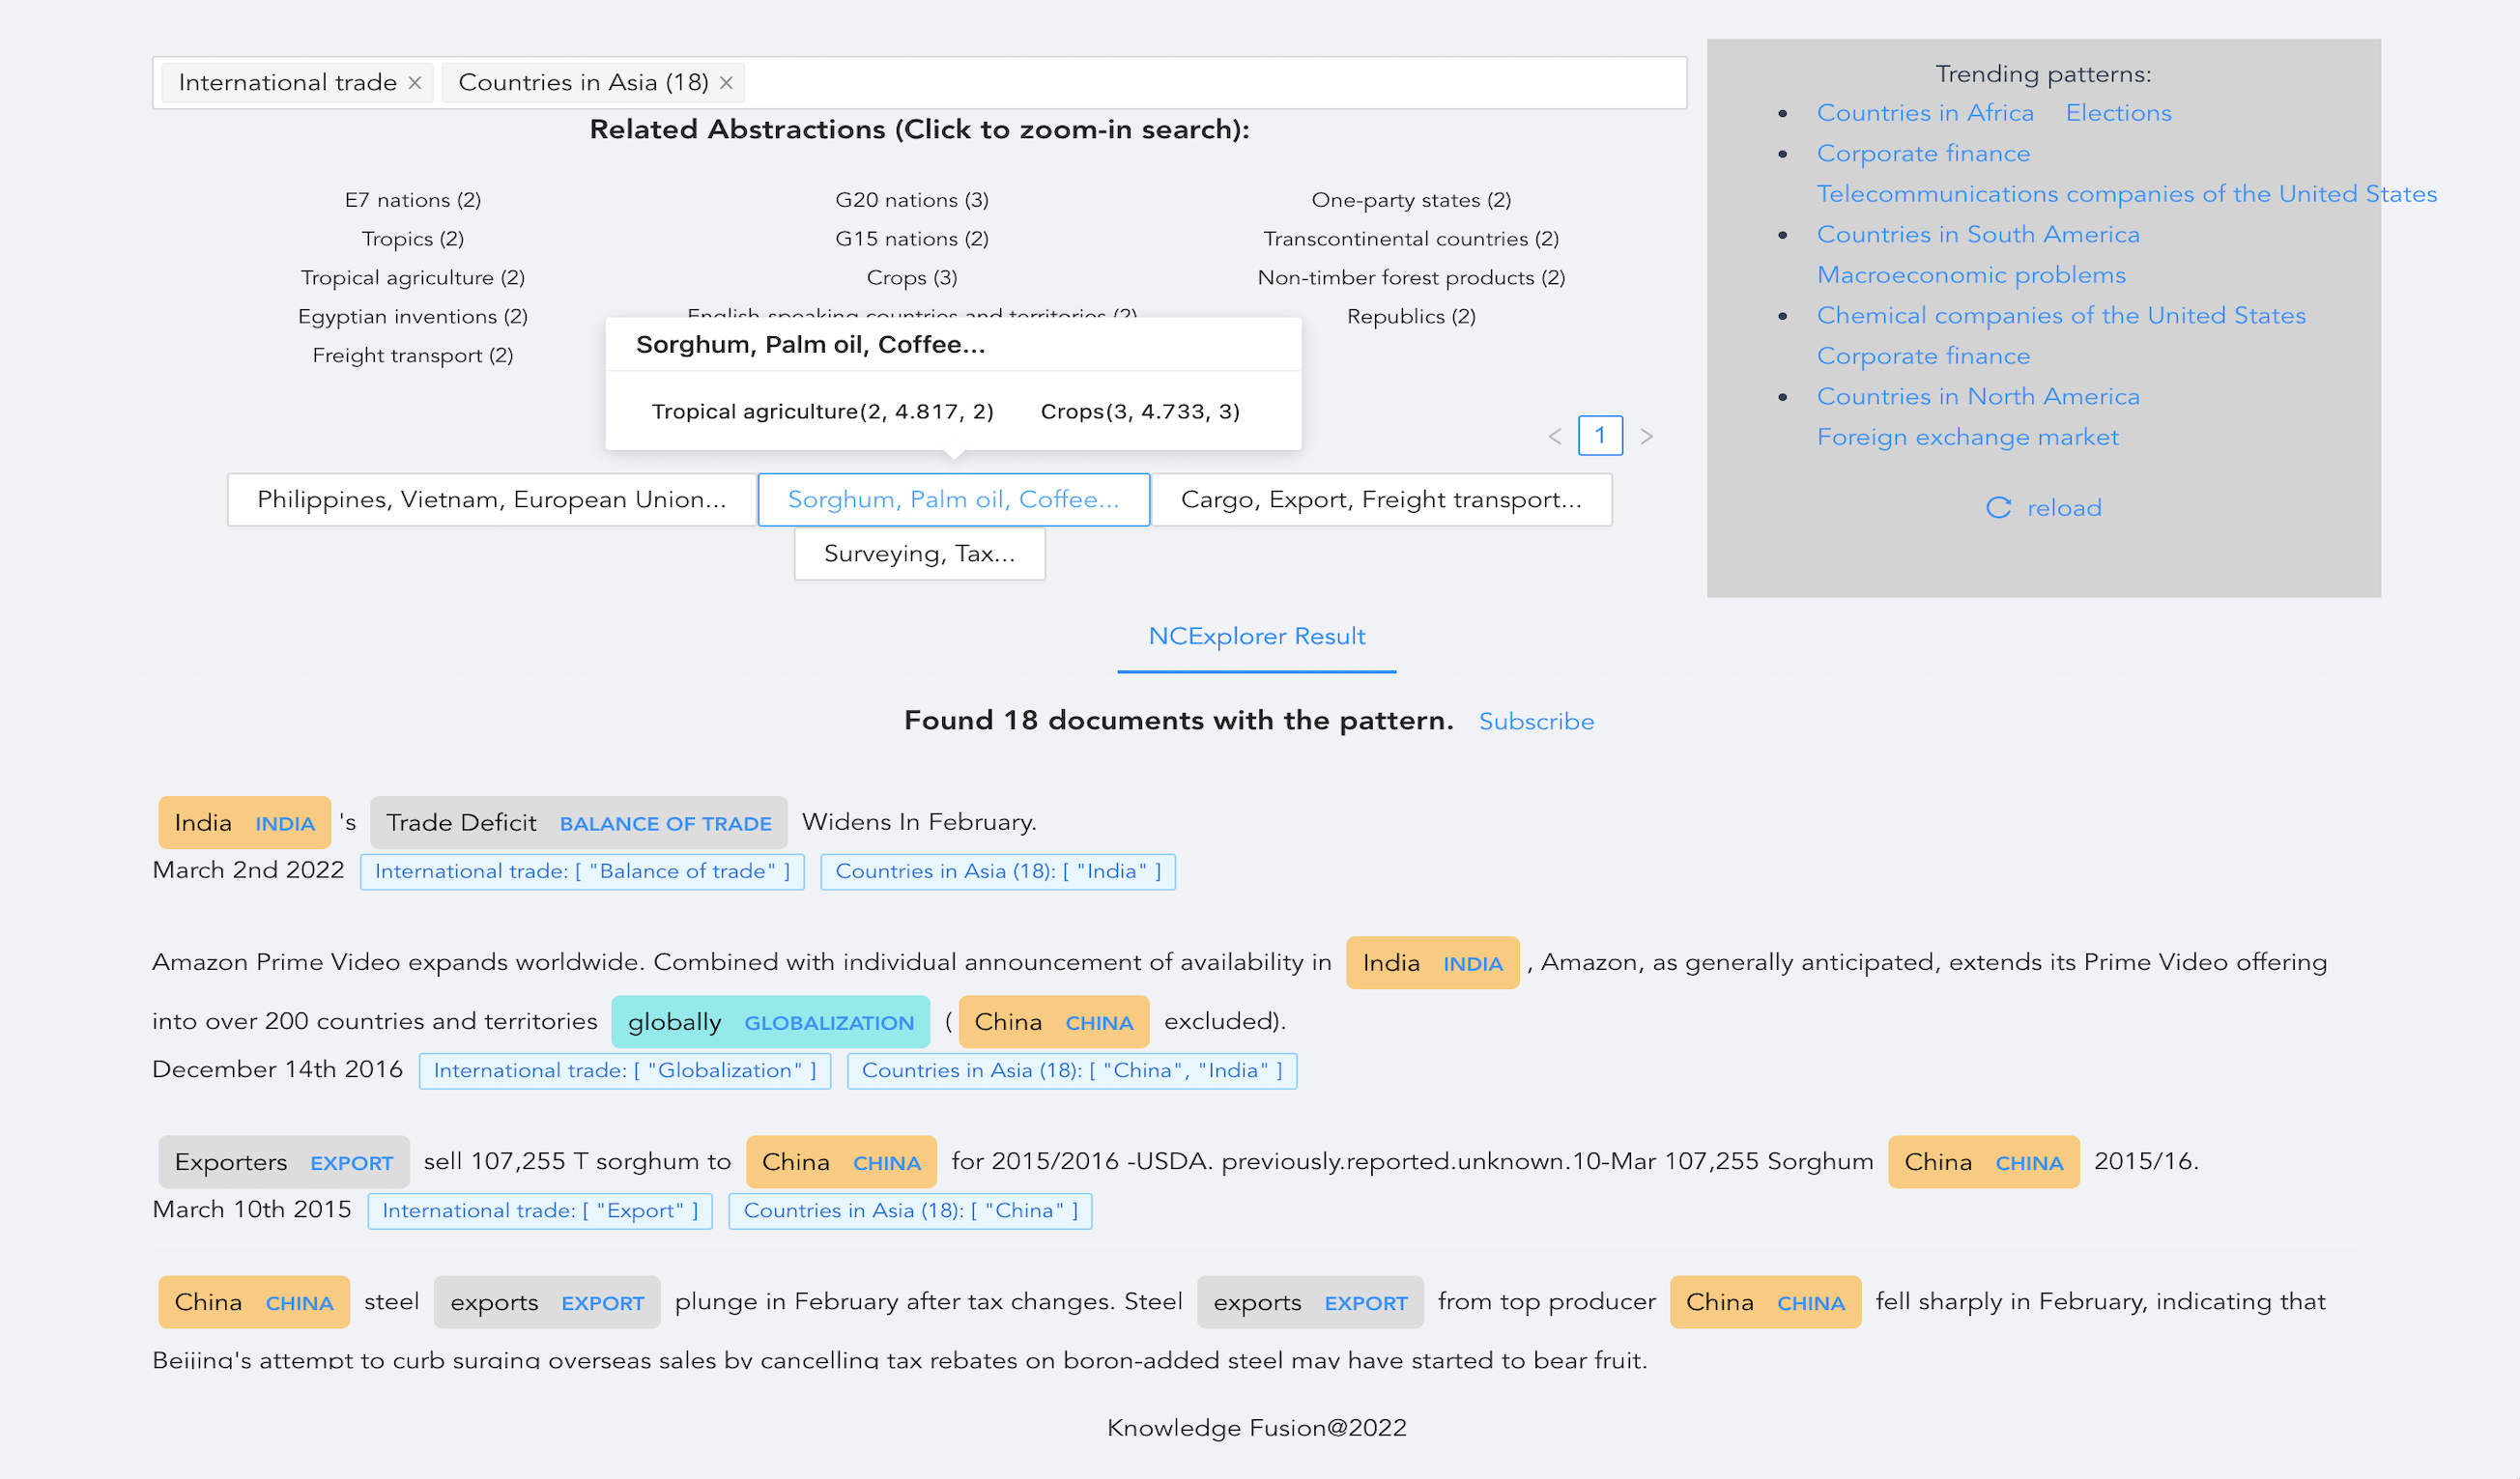}}\hfill
 \subfloat[topics subscription]
  {\includegraphics[width=.85\linewidth]{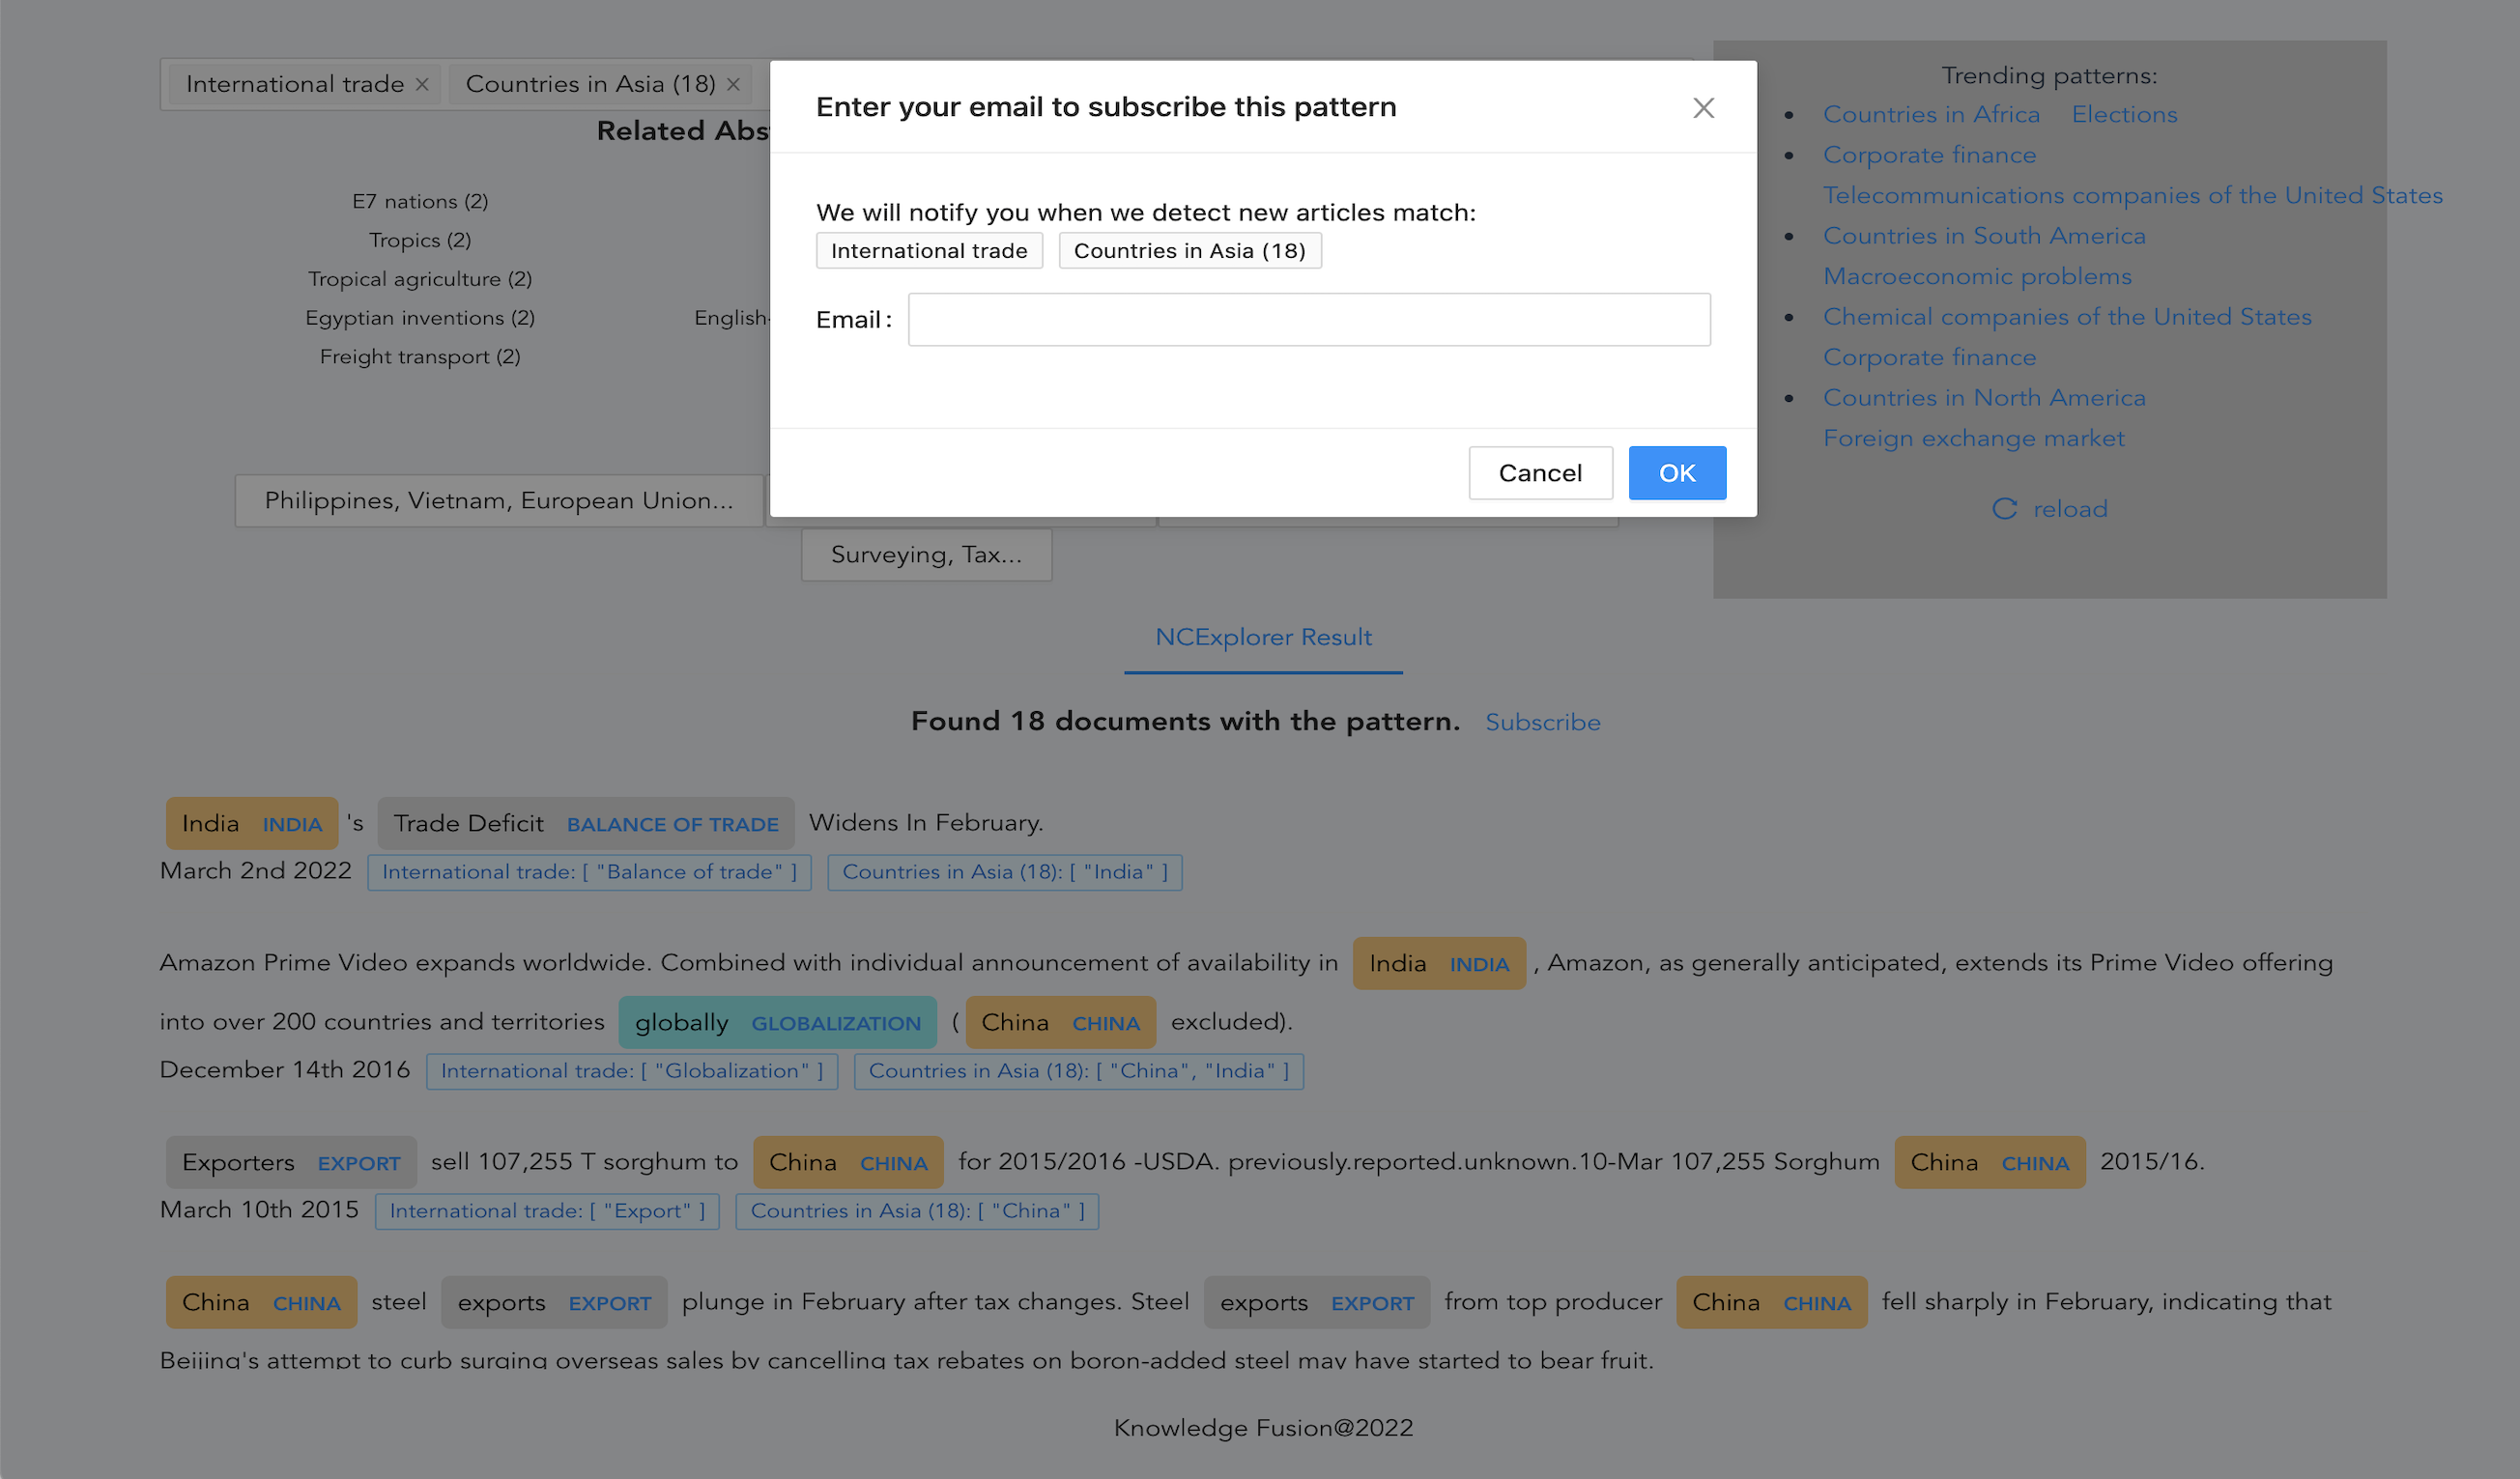}}\hfill
\caption{\framework search interface.}
  \label{fig:search-interface}

\end{figure*}

\begin{figure*}[ht]
\subfloat[select first concept]
  {\includegraphics[width=.85\linewidth]{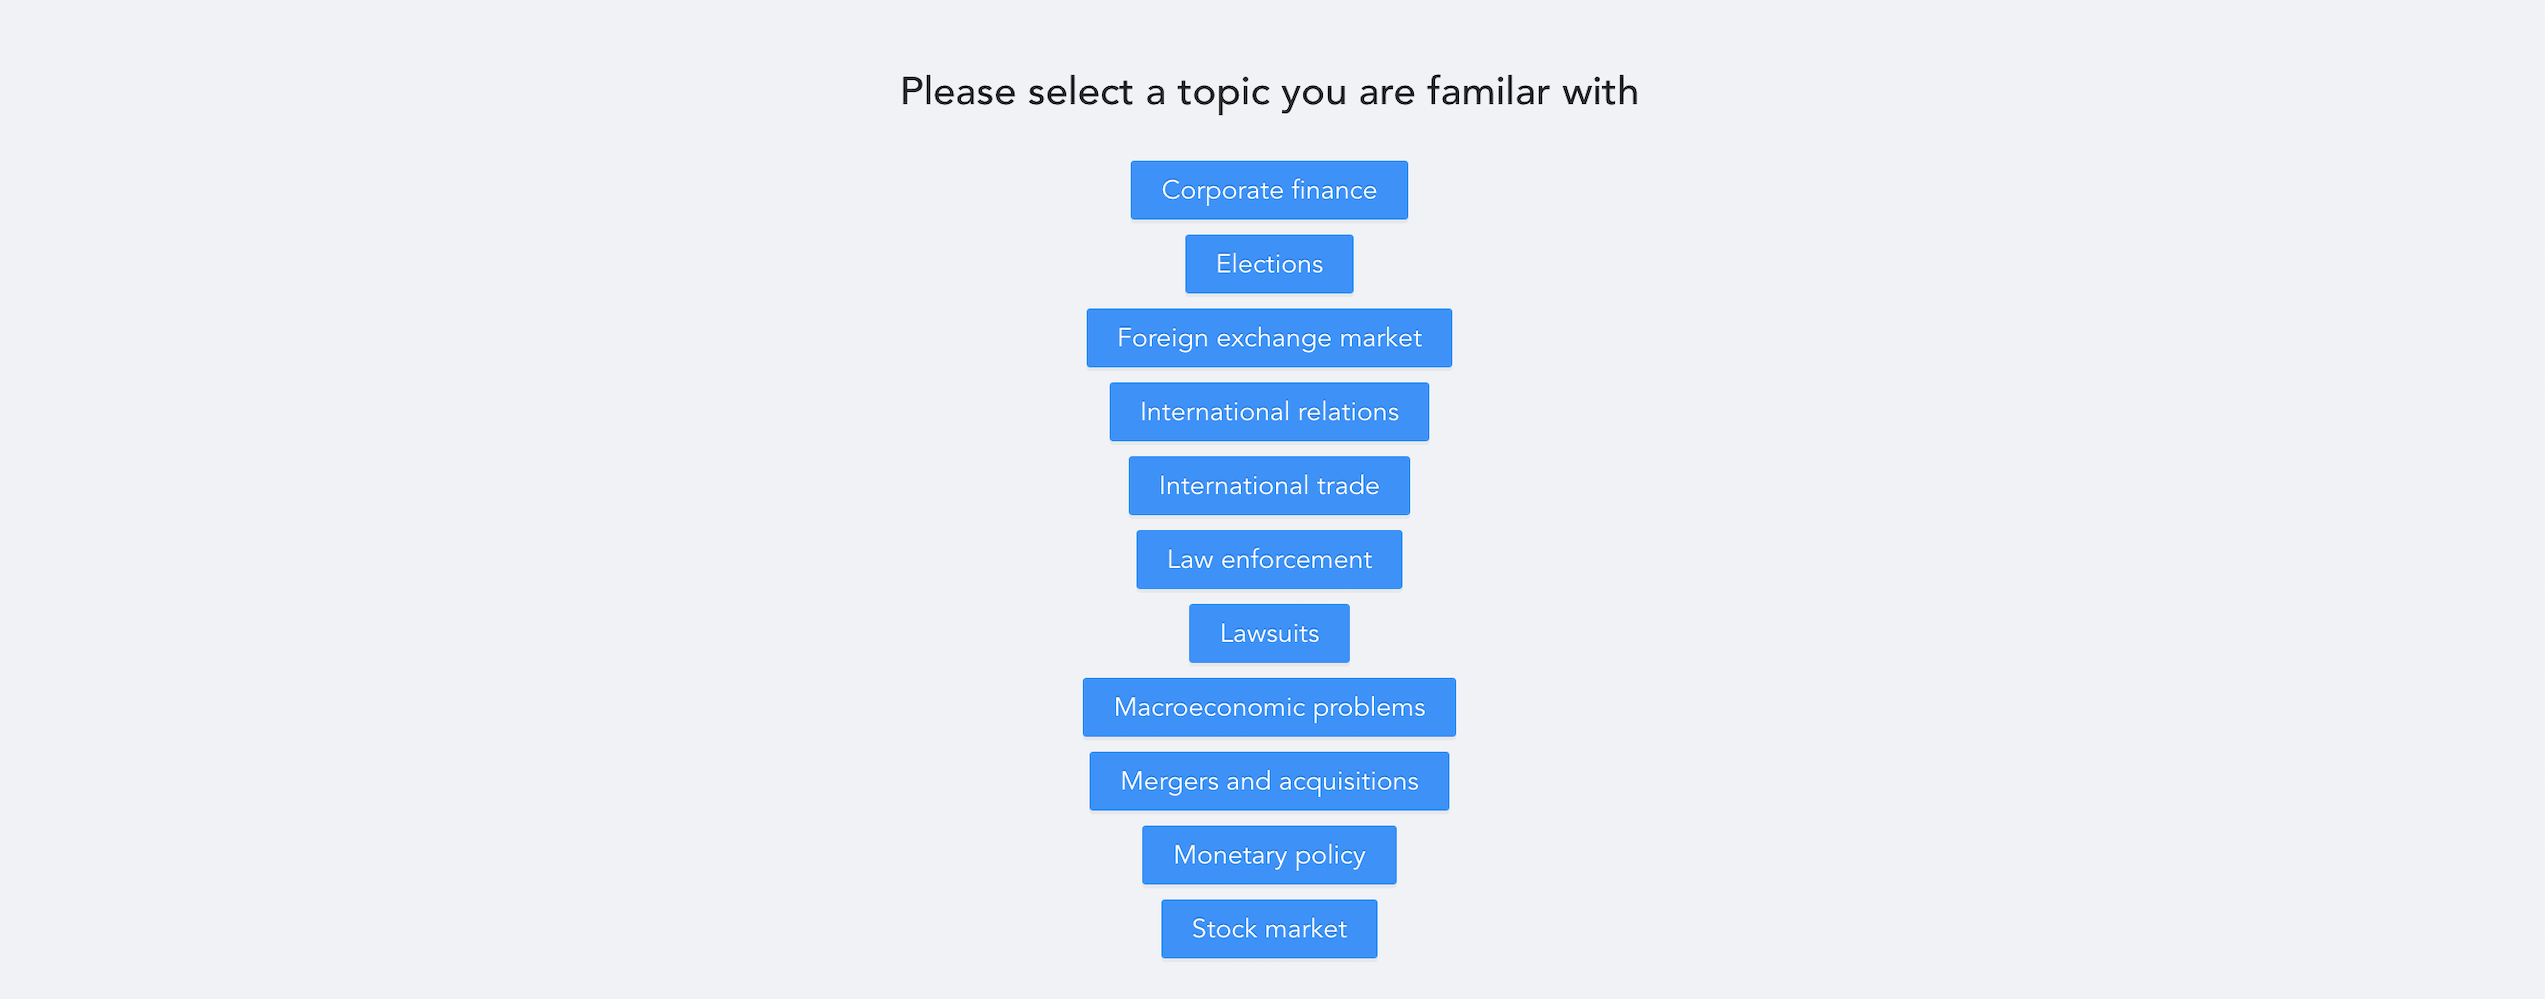}}\hfill
\subfloat[select second concepts]
  {\includegraphics[width=.85\linewidth]{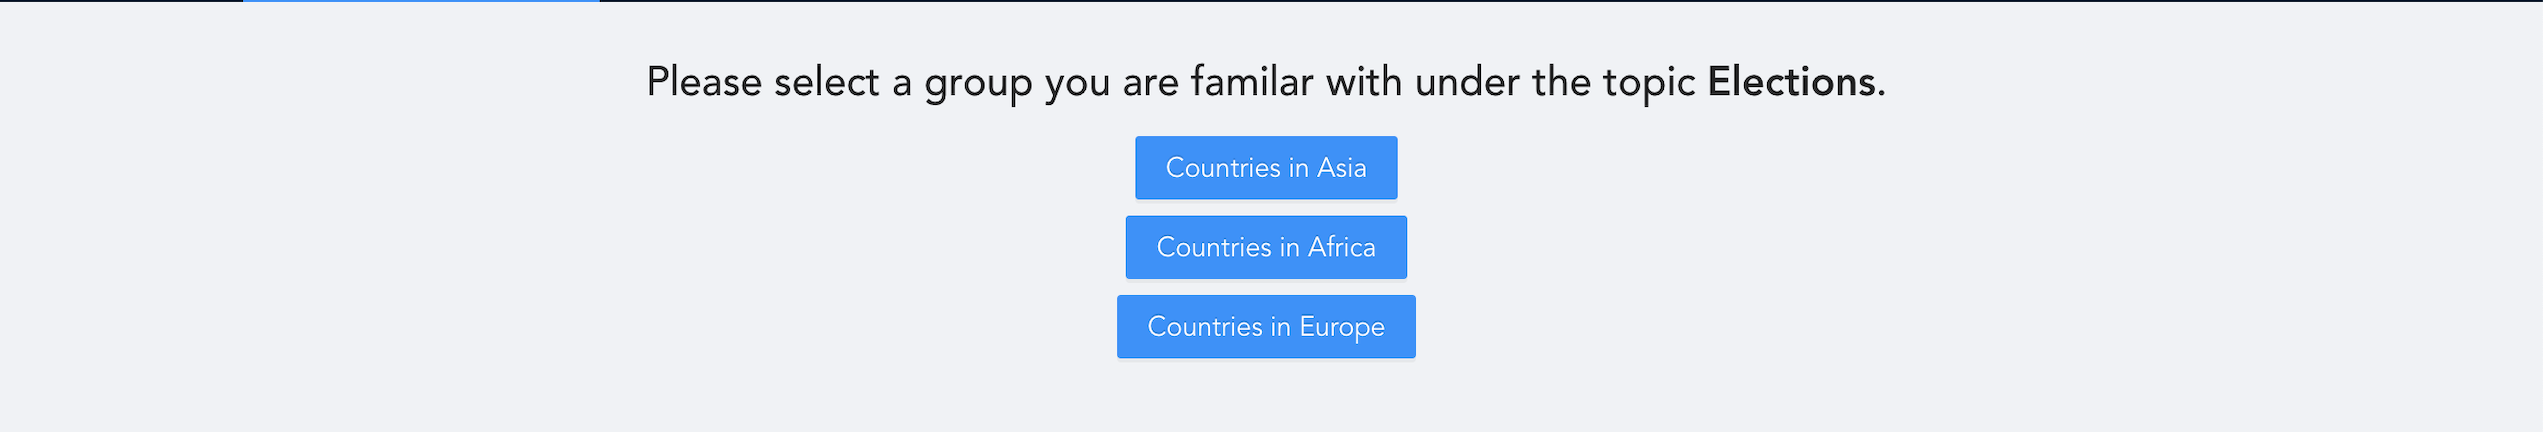}}\hfill
\subfloat[rate whether the document is relevant to \emph{both} concepts]
  {\includegraphics[width=.85\linewidth]{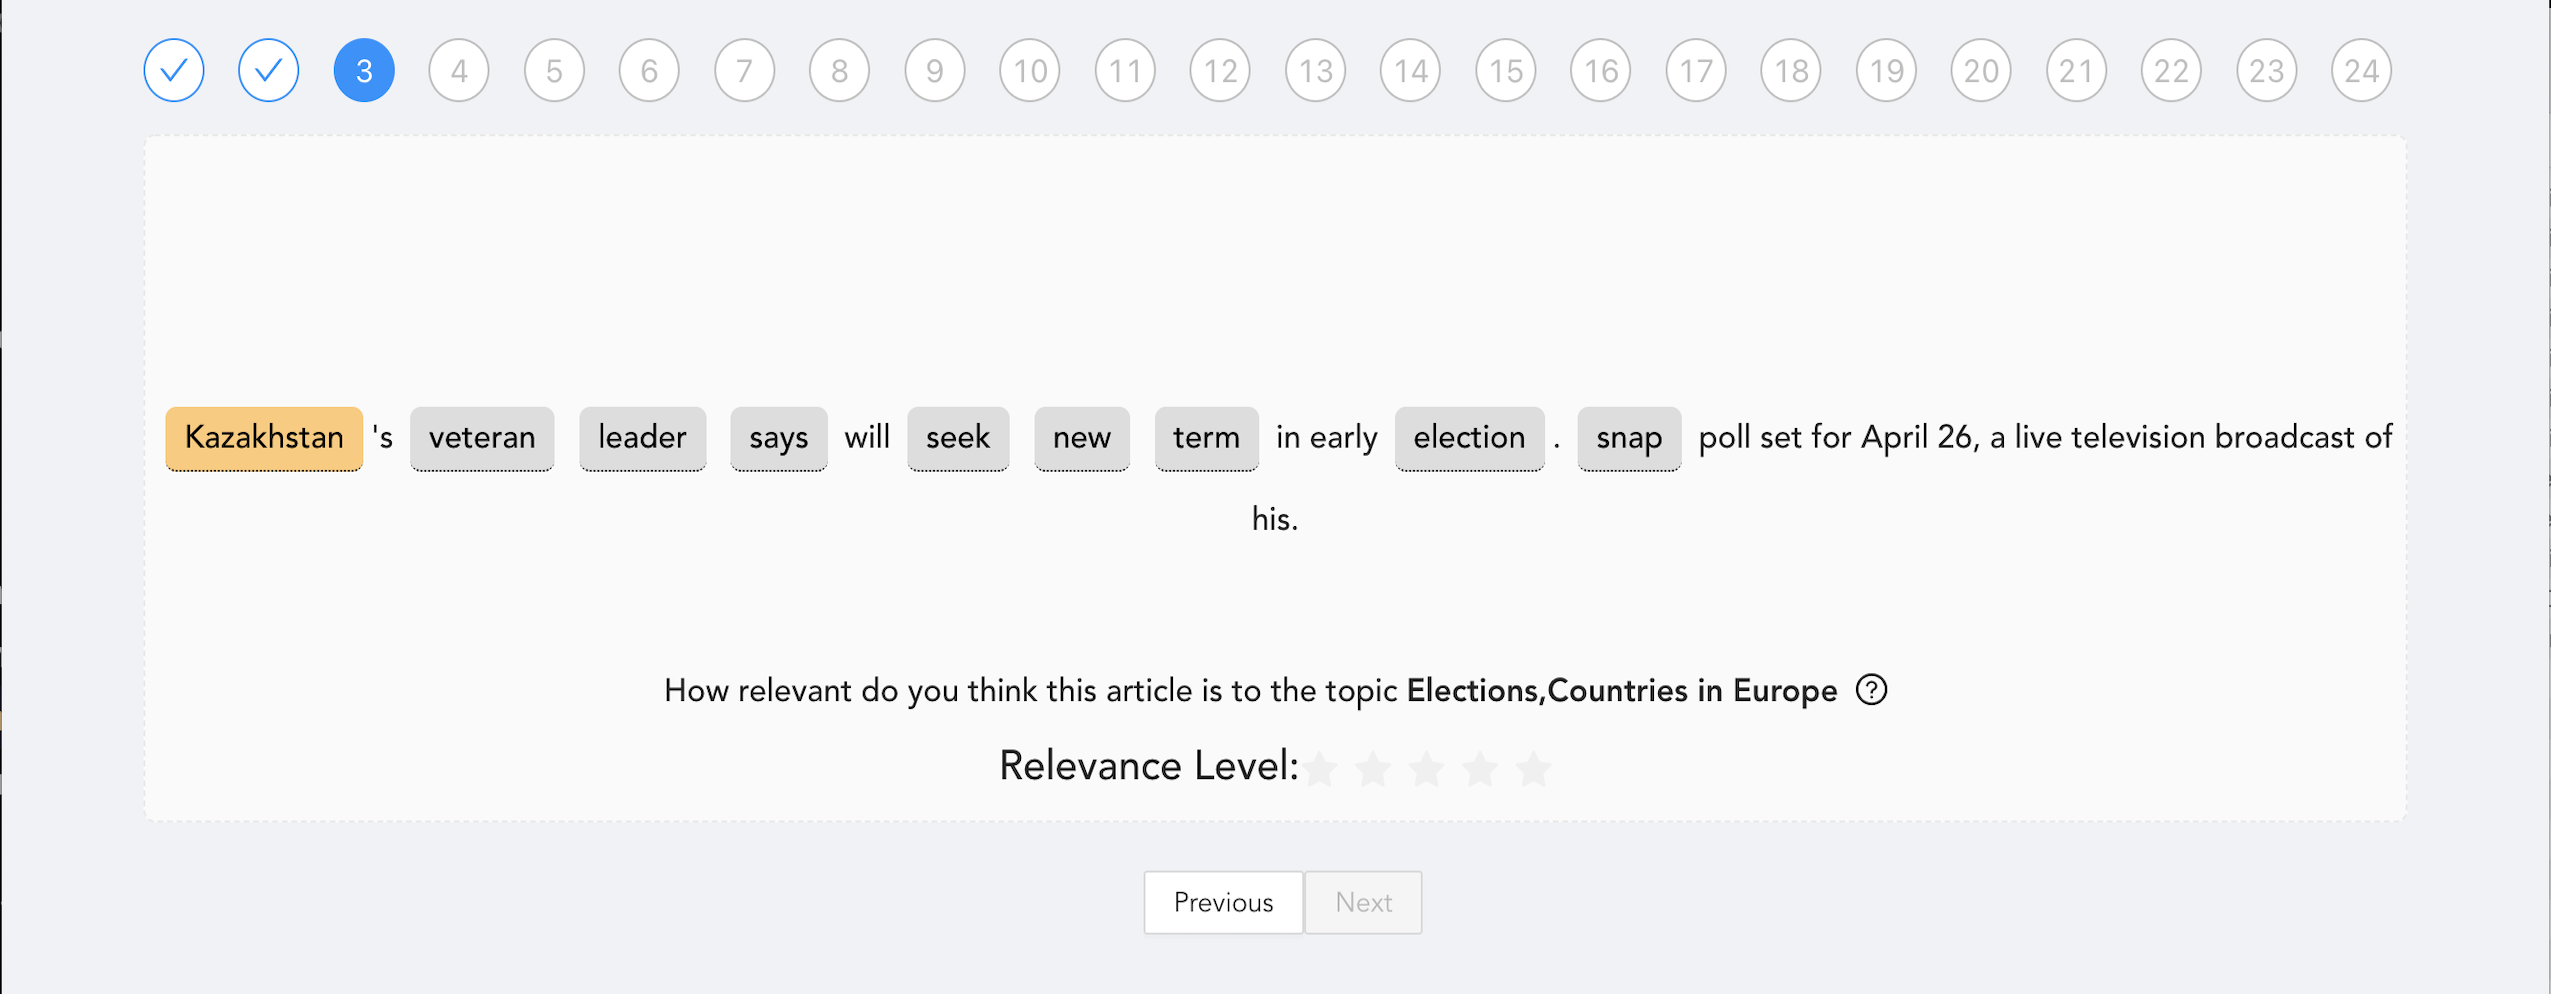}}\hfill
 \subfloat[one possible user rating]
  {\includegraphics[width=.85\linewidth]{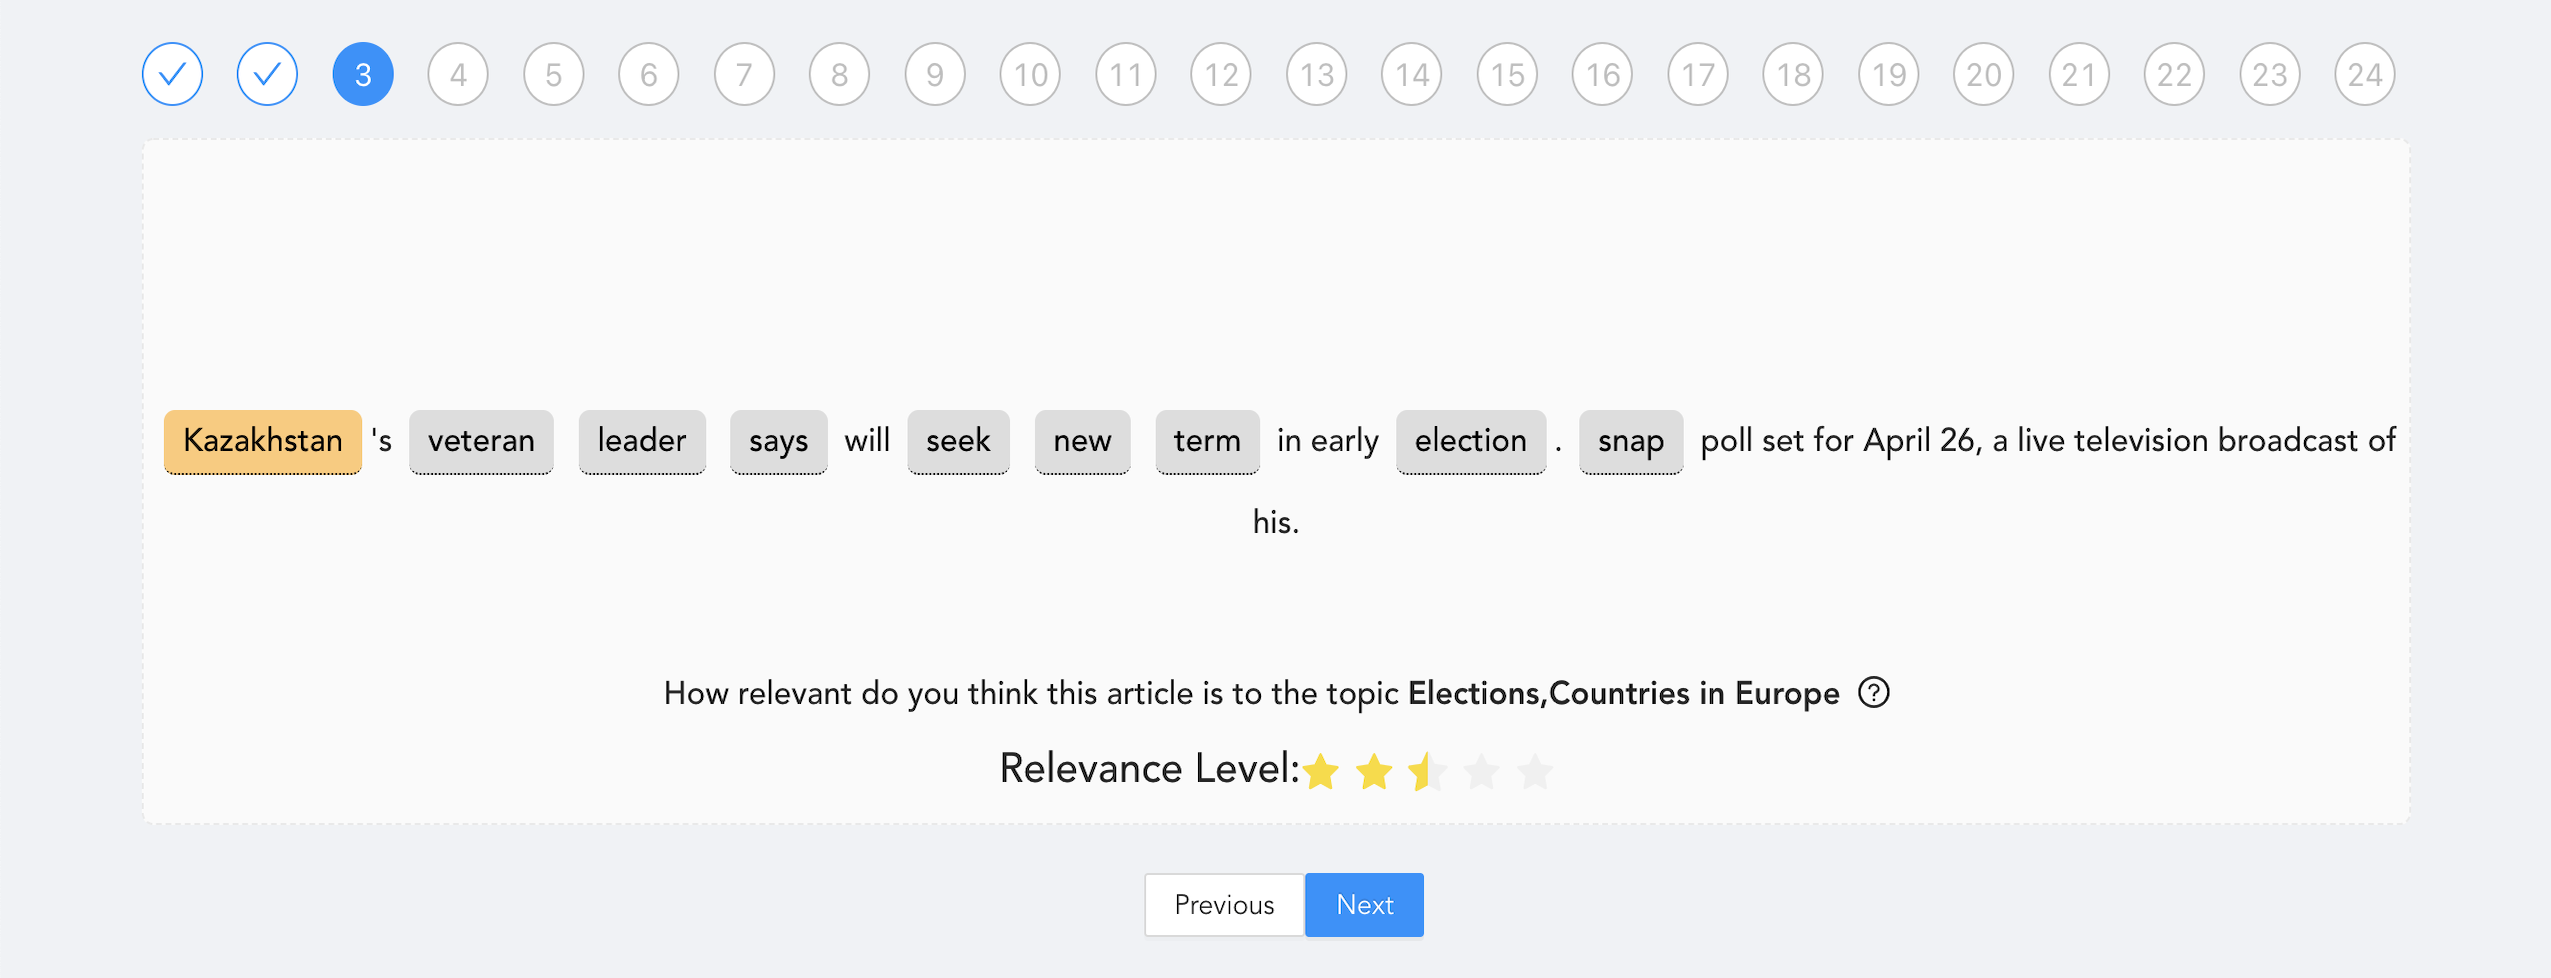}}\hfill
\caption{\framework Effectiveness Study Survey. Each participant is asked to select two concepts and rate 25 documents.}
  \label{fig:effectiveness_study_survey_interface}

\end{figure*}

\begin{figure*}[ht]
\subfloat[documents associated with first subtopic]
  {\includegraphics[width=.45\linewidth]{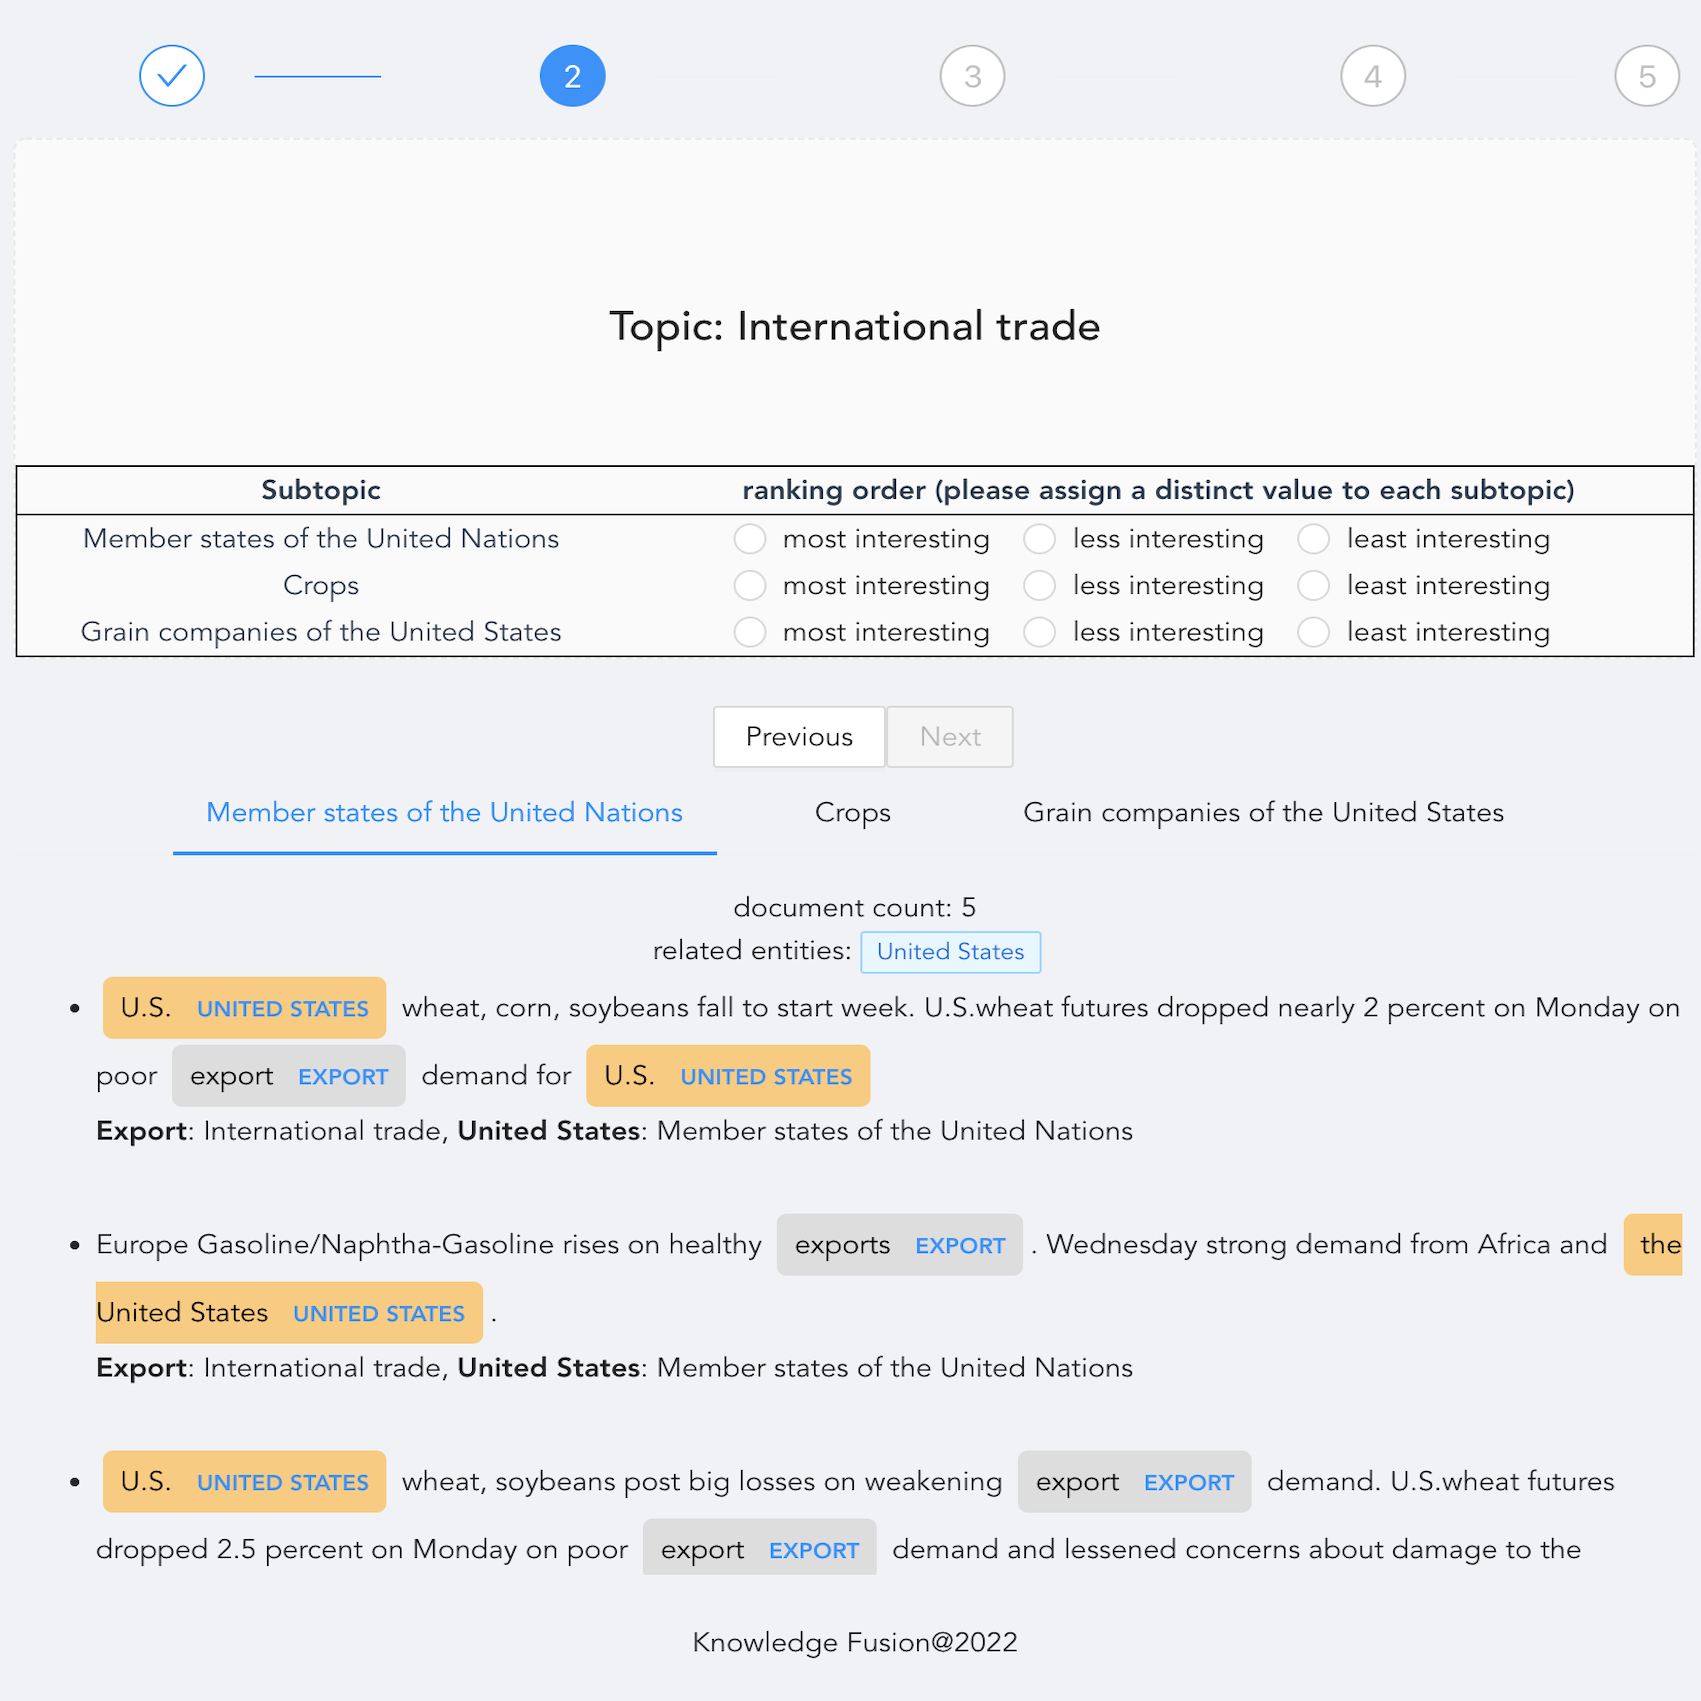}}\hfill
\subfloat[documents associated with second subtopic]
  {\includegraphics[width=.45\linewidth]{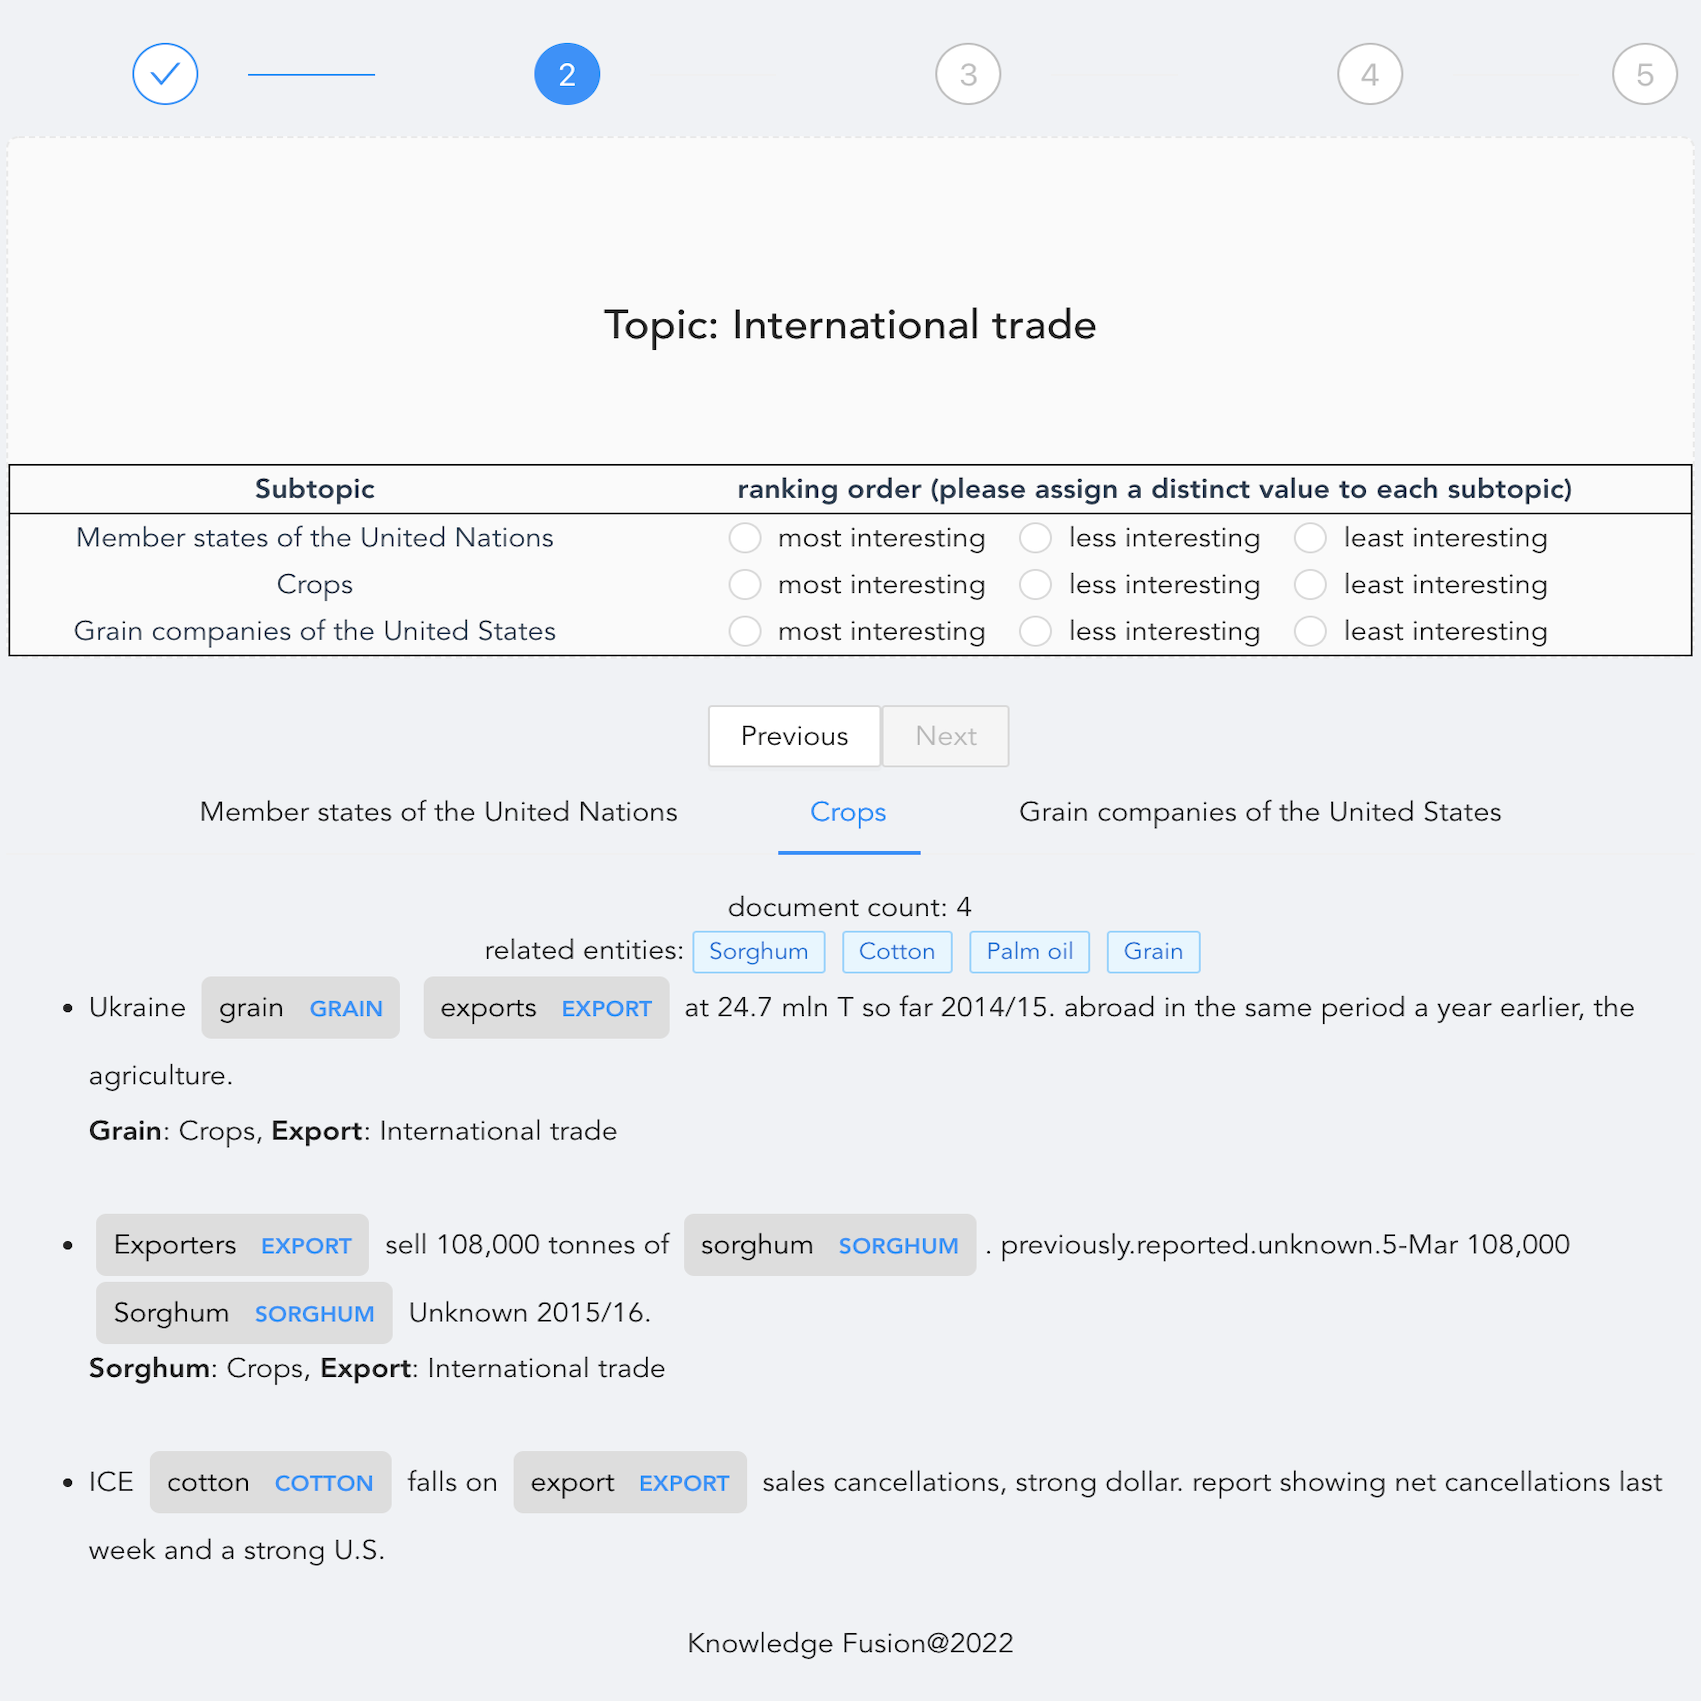}}\hfill
\subfloat[documents associated with third subtopic]
  {\includegraphics[width=.45\linewidth]{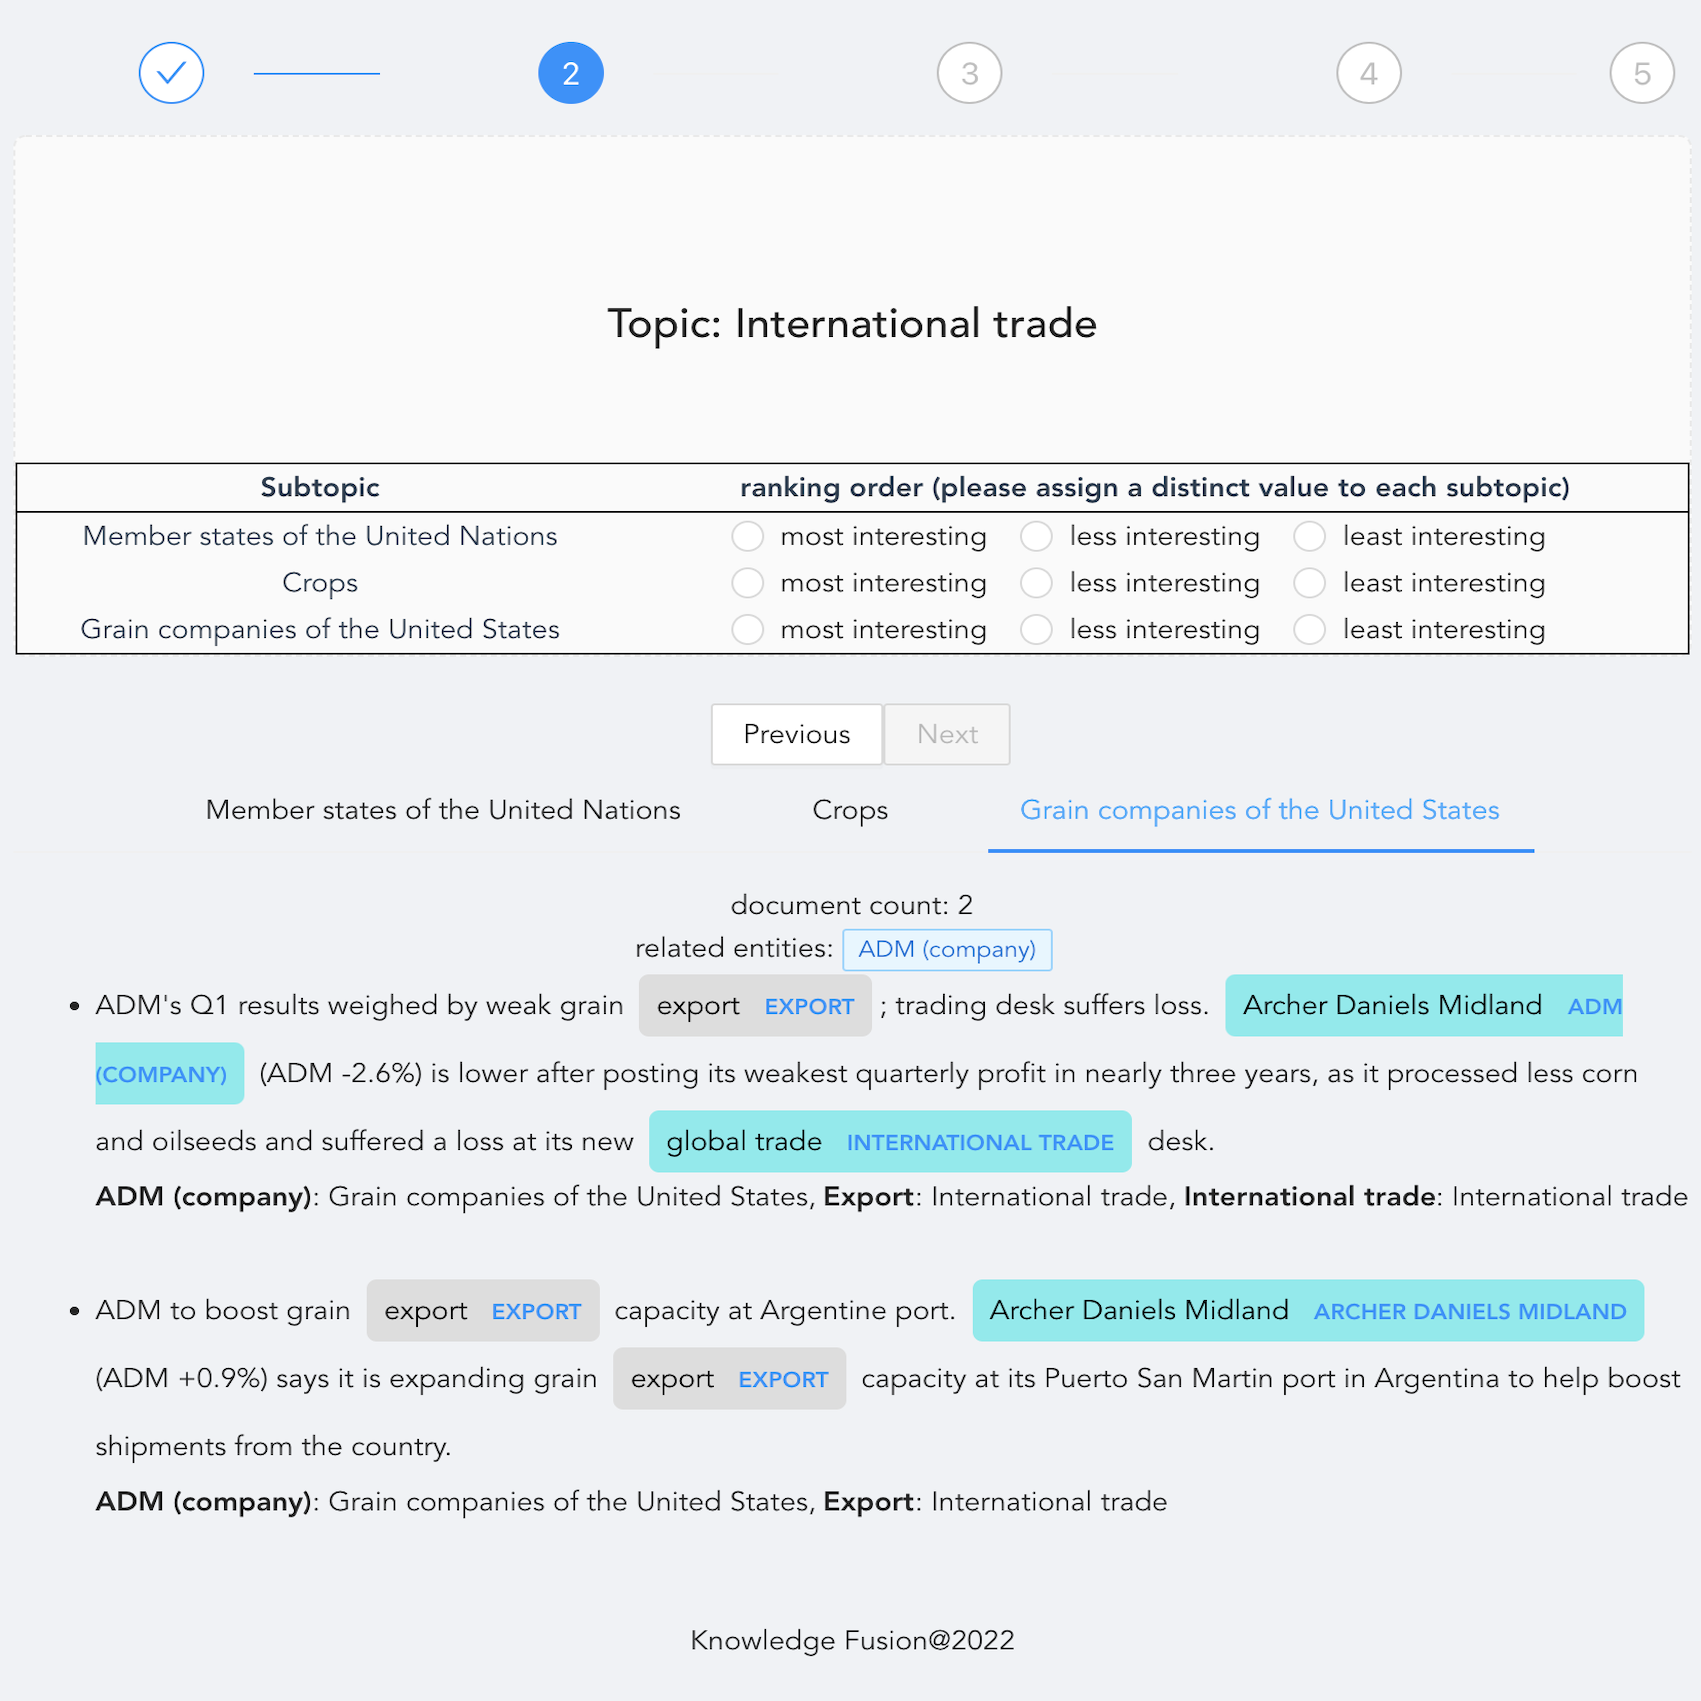}}\hfill
 \subfloat[one possible user rating]
  {\includegraphics[width=.45\linewidth]{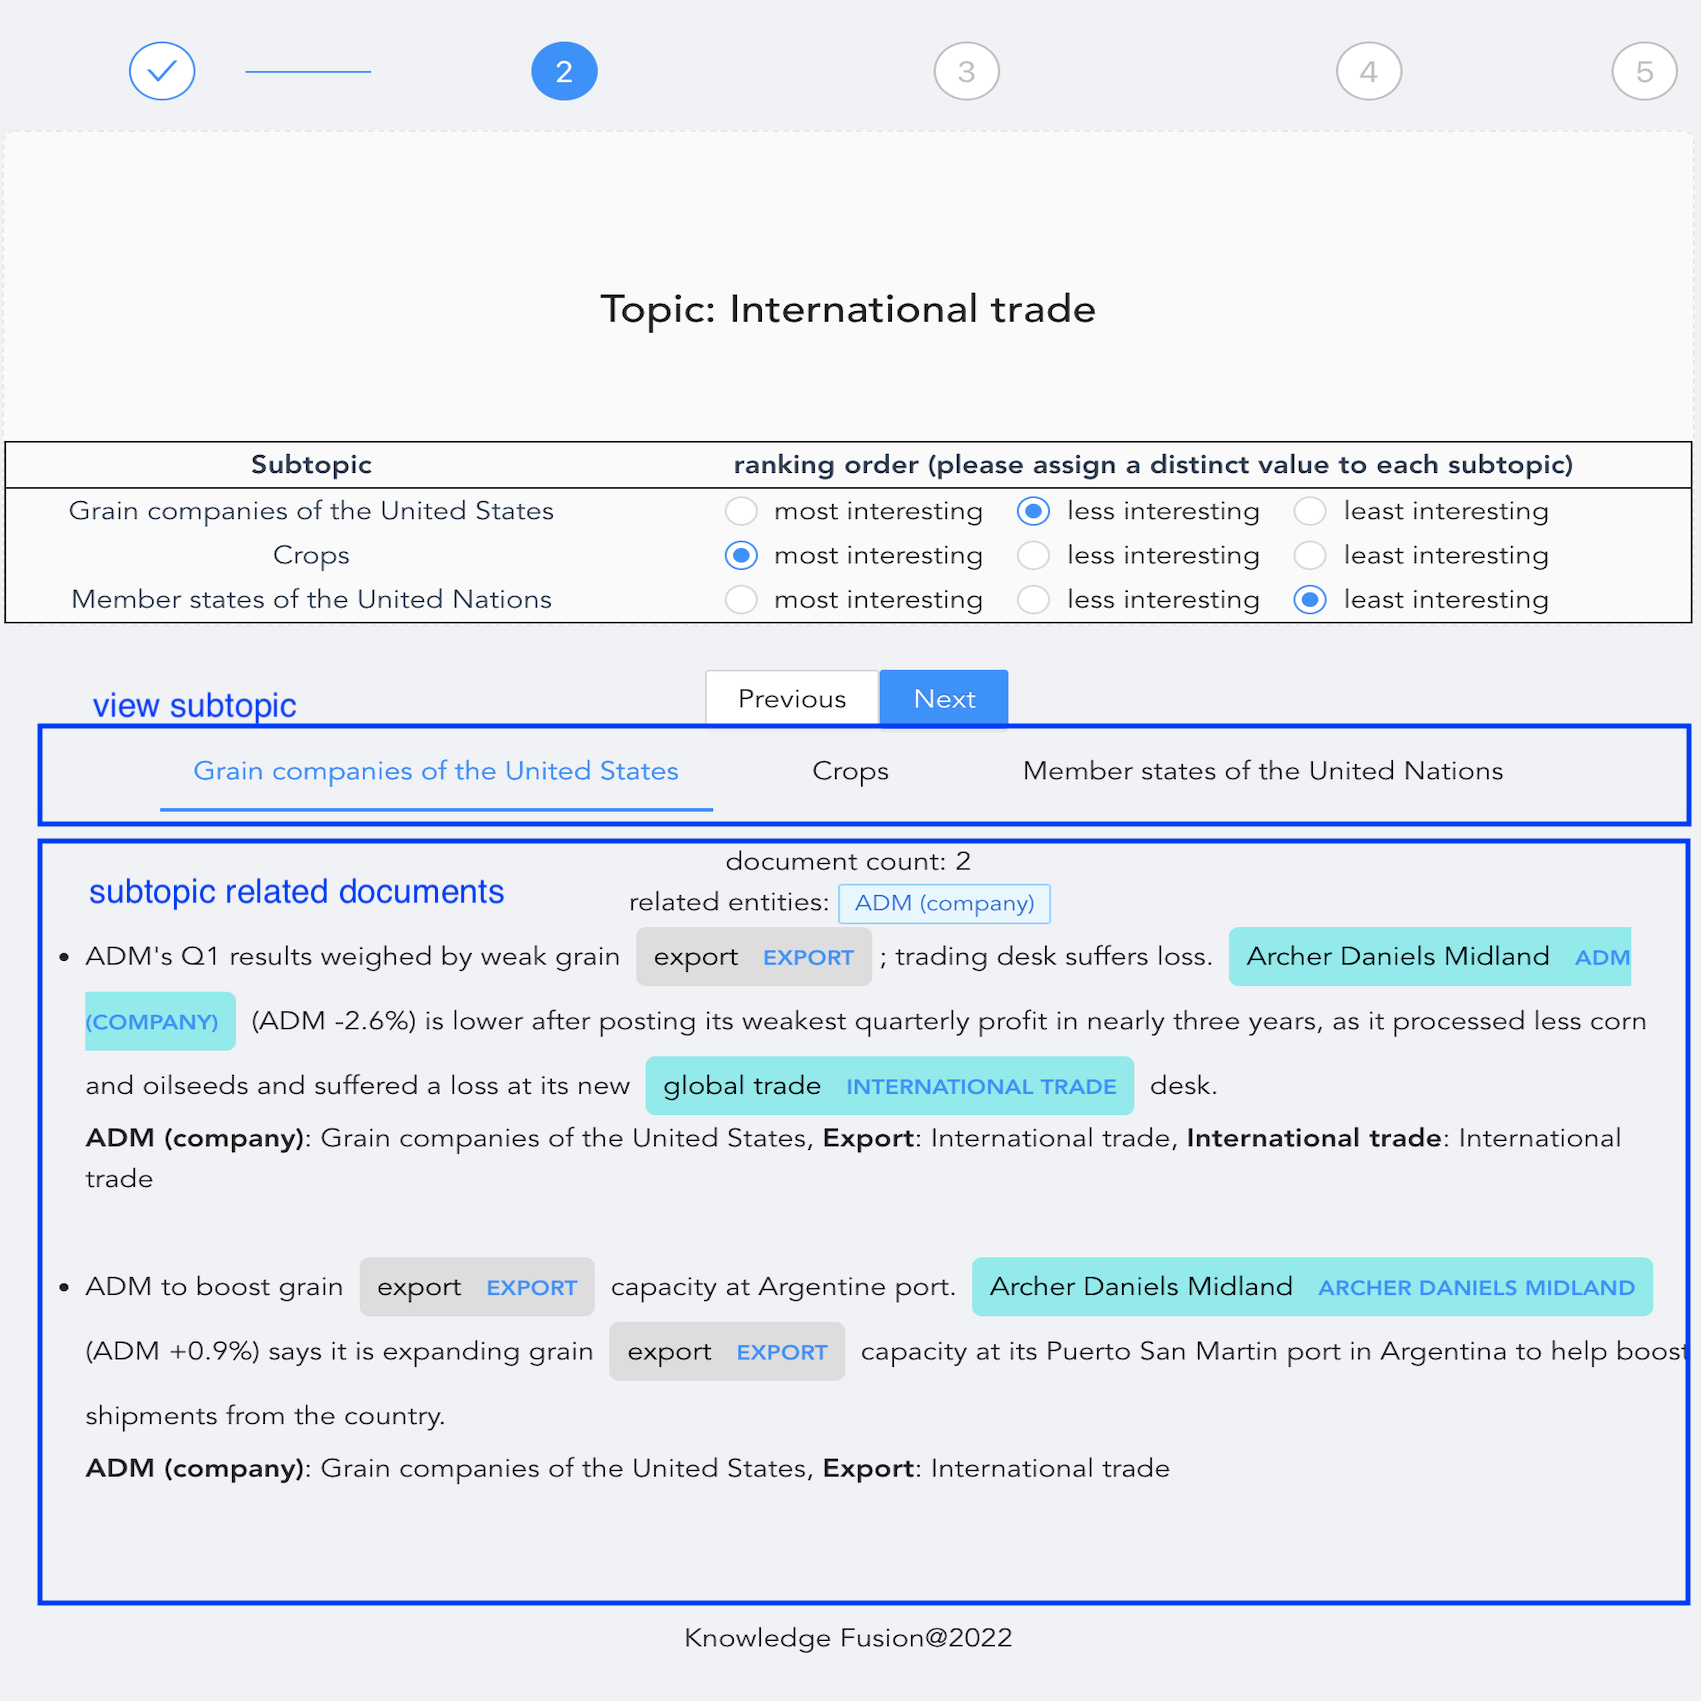}}\hfill
\caption{Subtopic Survey Interface. Each participant is asked to rate 5 topics. Each topic contains 3 subtopics.}
  \label{fig:subtopics_survey_interface}

\end{figure*}
