# Supplementary material for: Enabling Roll-up and Drill-down Operations in News Exploration with Knowledge Graphs for Due Diligence and Risk Management
Source: arXiv:2405.04929 source file (2024-05-08)
Supplement: Supplementary file 2 [file appendix.tex]

\subsection{Connectivity Score Calculation}
To calculate connectivity score, our sampling approach with the k-hop reachability index in Algorithm~\ref{algo:samplekhop}.
For each random walk, we first sample the source $u_1$ and the target $v$. 
Subsequently, we iteratively sample the next node $u_{l+1}$ by scanning the neighbors of $u_l$. With the help of the k-hop index, we first check if a neighbor $n$ can reach $v$ within the hop constraint of $\tau-l$ (Line \ref{alg:hop-constrain})
Then, we uniformly sample eligible neighbors by a Reservoir sampler, which only requires a single scan of the neighbors (Line \ref{alg:single-scan})
A random walk terminates when either the target $v$ is sampled or the hop limit is reached.

\begin{table*}[h!]
\centering
  \caption{Extra Case Studies}
  
\begin{adjustbox}{width=1\linewidth}

\begin{tabular}{ |p{1.7cm}|p{1.7cm}|p{3cm}|p{10cm}|} 
    \hline
   Query & Roll-up options & Drill-down options & Results\\
   \hline
   \textcolor{teal}{Asian Countries}, \newline \textcolor{orange}{Stock Market} & \textcolor{orange}{Financial Markets} & Forex Market, \newline  National Oil and Gas Companies & 
   \vspace{-2mm}
   \begin{enumerate}
       \item \textcolor{teal}{Indonesia} Mining \textcolor{orange}{IPO} Vaults Six Shareholders to Billionaire Status 
       \item \textcolor{teal}{China} Tightens Oversight of Program Trading in \textcolor{orange}{Stock Market}
       \item TY Fashion, a Taiwanese-owned garment manufacturer in \textcolor{teal}{Cambodia}, has received approval for listing on the Cambodia \textcolor{orange}{Securities Exchange}
   \end{enumerate}
   \vspace{-3mm}
  \\ \hline
  \textcolor{teal}{Biotechnology Companies of the U.S.}, \newline \textcolor{orange}{M\&A} & \textcolor{orange}{Corporate Finance} & Orphan Drug Companies, \newline Multinational Food Companies &
  \vspace{-2mm}
    \begin{enumerate}
        \item Unilever has expressed interest in acquiring \textcolor{teal}{GlaxoSmithKline}'s consumer healthcare business, a \textcolor{orange}{joint venture} with Pfizer.
        \item  \textcolor{teal}{GSK} leads race to \textcolor{orange}{buy} \textcolor{teal}{Pfizer} unit.
        \item  \textcolor{teal}{Pfizer} to \textcolor{orange}{Purchase} Cancer Drugmaker \textcolor{teal}{Seagen} for \$43 Billion
    \end{enumerate}
    \vspace{-3mm}
  \\ \hline
  \textcolor{teal}{EU countries}, \newline \textcolor{orange}{Labor Disputes} & \textcolor{orange}{social conflicts} & Minimum Wage & 
   \vspace{-2mm}
    \begin{enumerate}
    \item Protesters in \textcolor{teal}{France} demonstrate against President Emmanuel Macron's pension overhaul and the end of the longest transport \textcolor{orange}{strike} in French history.
    \item  \textcolor{teal}{Greece}'s leftist government plans to raise the minimum wage and restore \textcolor{orange}{collective bargaining}, as it seeks to renegotiate the terms of its international bailout
    \item  Amazon faces \textcolor{orange}{strike} of logistical workers in \textcolor{teal}{Germany}
       \end{enumerate}
    \vspace{-3mm}
    \\
 \hline
 \textcolor{teal}{Investment Banks},  \textcolor{orange}{Commercial Crimes} & \textcolor{orange}{Corporate Crimes} & Hedge Funds, \newline  Online Brokerages, \newline Investment Funds, \newline Interest Rates &
 \vspace{-2mm}
    \begin{enumerate}
    \item Broker Faces \textcolor{orange}{Insider Trading} Probe Tied to \textcolor{teal}{Morgan Stanley} Deals.
    \item  Ex-\textcolor{teal}{Morgan Stanley} Adviser Gets Seven Years for Fleecing Clients in \textcolor{orange}{Ponzi Scheme}.
    \item \textcolor{teal}{Deutsche Bank} Said to Probe Senior Russia Employee Over \textcolor{orange}{Bribes}.
    \item \textcolor{teal}{UBS} has lost its appeal against a French \textcolor{orange}{tax evasion} charge.
    \item  \textcolor{teal}{JPMorgan} fined for \textcolor{orange}{wash trades} in oil, gasoline
       \end{enumerate}
    \vspace{-3mm}
    \\ \hline
\end{tabular}
\end{adjustbox} 
  \label{tab:extra-case-studies}
\end{table*}

\begin{algorithm2e}
   % \LinesNumbered
	\SetKwInOut{Input}{Input}
	\SetKwInOut{Output}{Output}
	\Input{KG $\mathcal{G}$, concept $c$, document $d$, sample size $\theta$}
	\Output{the estimated connectivity $est$}
        $est \gets 0$; \\
	\While{there are less than $\theta$ random walks}{
		  $l \gets 1$; $p \gets 1.0$; \\
		  $u_l \gets$ a random entity in $\onto(c)$; \\
		  $v \gets$ a random entity in $CE(c,d)$; \\
		  \While{$l \leq \tau$}{
			$count \gets 0$; \\ 
			\ForEach{$n \in N(u_l)$}{
				\If{$hop(n,v) \leq \tau-l$ \label{alg:hop-constrain}}{
					$count \gets count + 1$; \\
					$u_{l+1} \gets n$ with probability $\frac{1}{count}$;\label{alg:single-scan}
				}				
			}
			$p \gets \frac{p}{count}$; \\
			$l \gets l+1$; \\
			\textbf{break} on $u_{l} = v$; 
		}
		\If{$u_{l} = v$}{
			$est \gets est + \frac{\beta^{l-1}}{p}$;
		}
	}
	\Return {$\frac{est \cdot |\onto(c)|}{\theta} $.} \\
	\caption{Random walk estimator with k-hop index.} 
	\label{algo:samplekhop}
\end{algorithm2e}

\subsection{Survey Interface}
To assess the effectiveness of our connectivity score and to understand the impact of different subtopics ranking, we have developed interactive interfaces, as shown in Figures ~\ref{fig:effectiveness_study_survey_interface} and ~\ref{fig:subtopic-survey-interface}, respectively. These interfaces allow users to visually explore how the connectivity score and subtopics ranking contribute to the overall performance of our system.

\subsection{Extra Case Studies}
In addition to these interactive studies, we have compiled a range of case studies spanning various topics in Table ~\ref{tab:extra-case-studies}. These case studies further exemplify the versatility and robustness of our approach in handling diverse content.

Furthermore, Figure ~\ref{fig:results-with-sentiment} provides a glimpse into the sentiment analysis aspect of our system. It depicts the varied sentiments associated with the purchase of \kgentity{Mass media in the United States} by \kgentity{American billionaires}, showcasing our system's ability to extract and analyze sentiment from news articles, which can be particularly useful for understanding public opinion and media portrayal of specific events or transactions.
\begin{figure}
\centering
\begin{adjustwidth}{}{}
    \begin{minipage}{\linewidth}
        {\includegraphics[width=\linewidth]{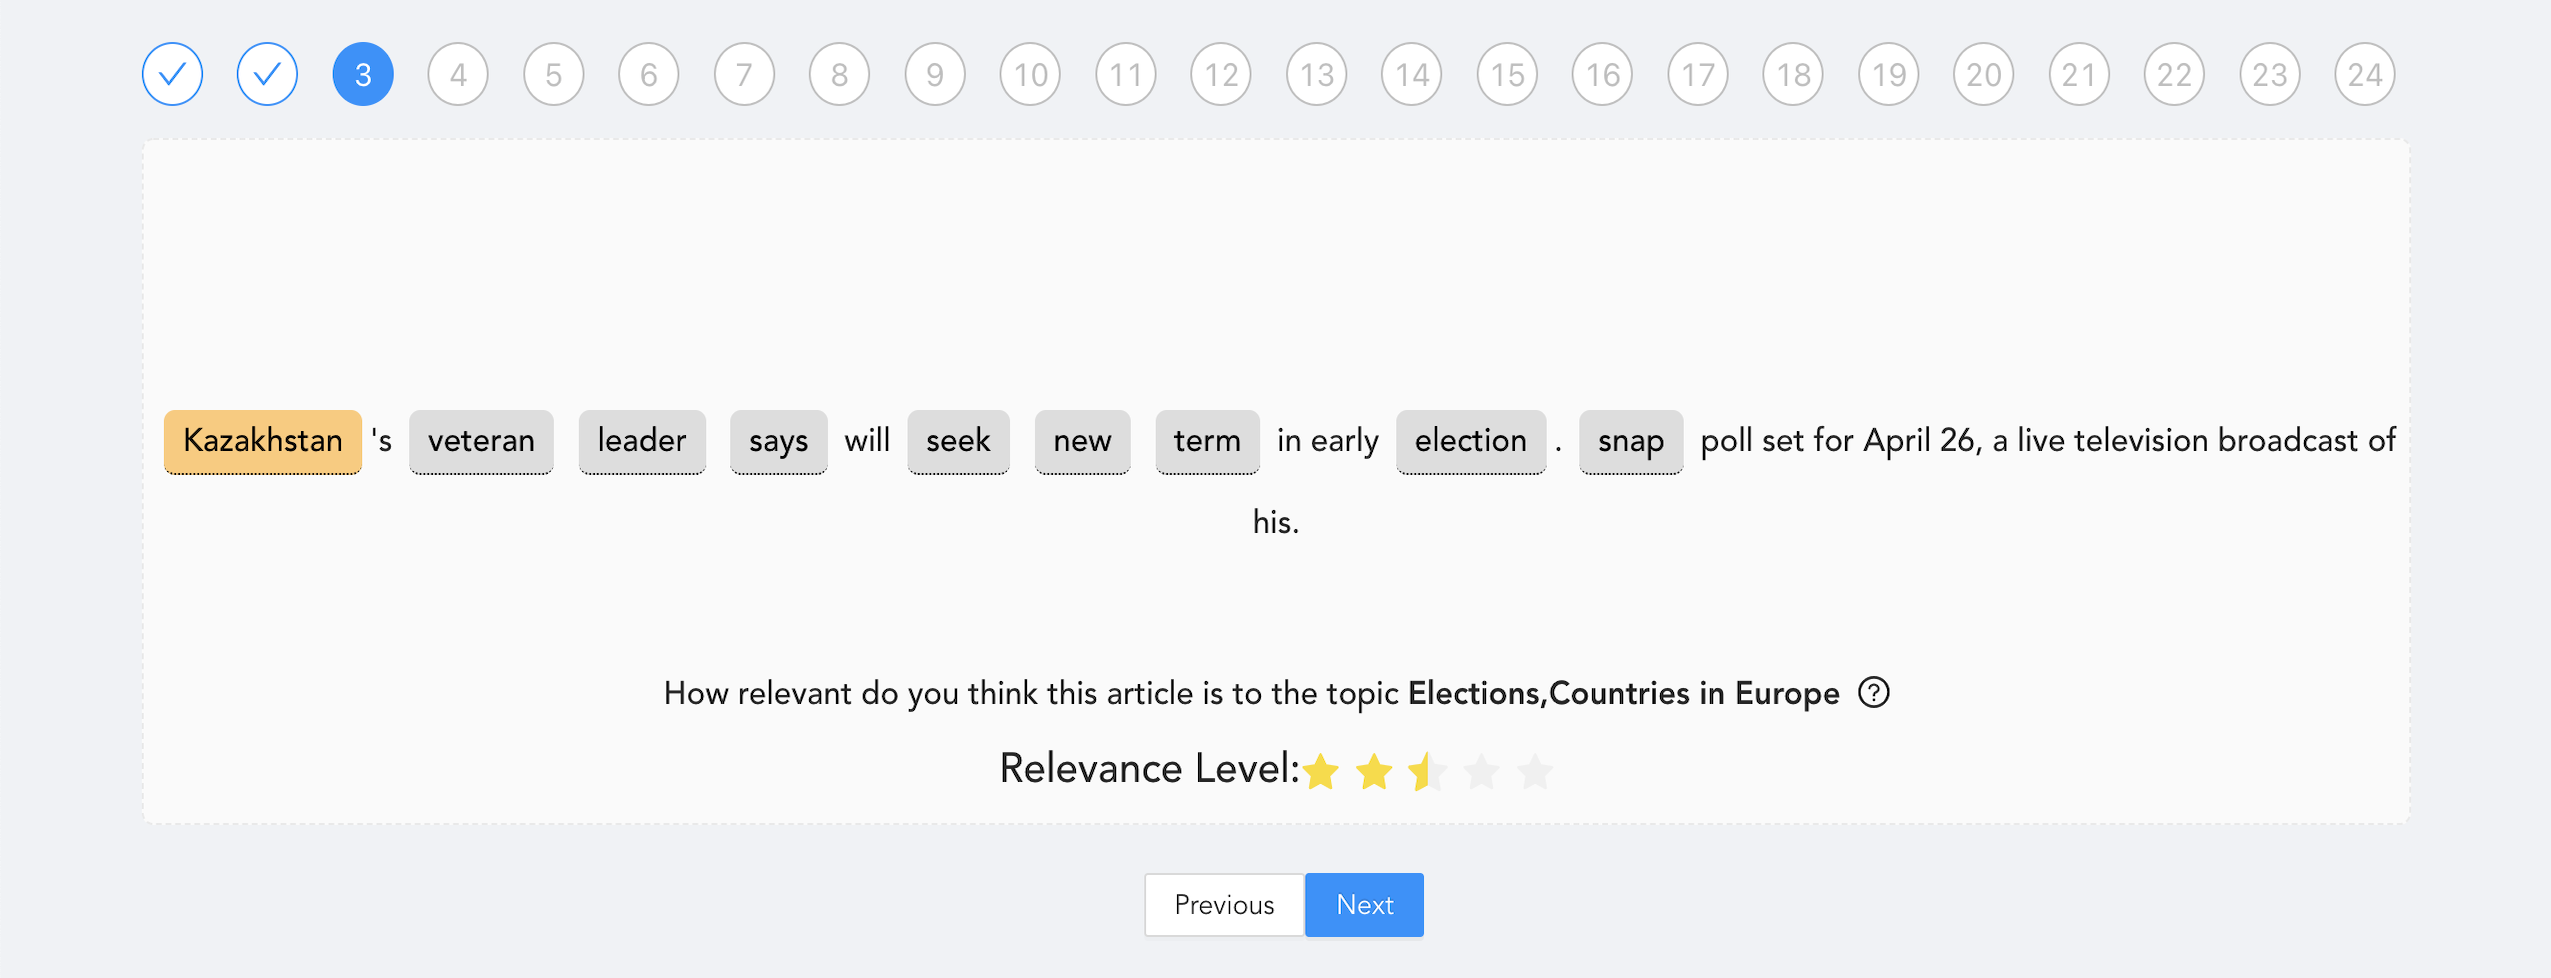}}\hfill
        \caption{Concept document relevance study survey interface. Each participant is asked to select two concepts and rate 25 documents.}
    \label{fig:effectiveness_study_survey_interface}
    \end{minipage}
    \begin{minipage}{\linewidth}
        \centering
        \includegraphics[width=\textwidth]{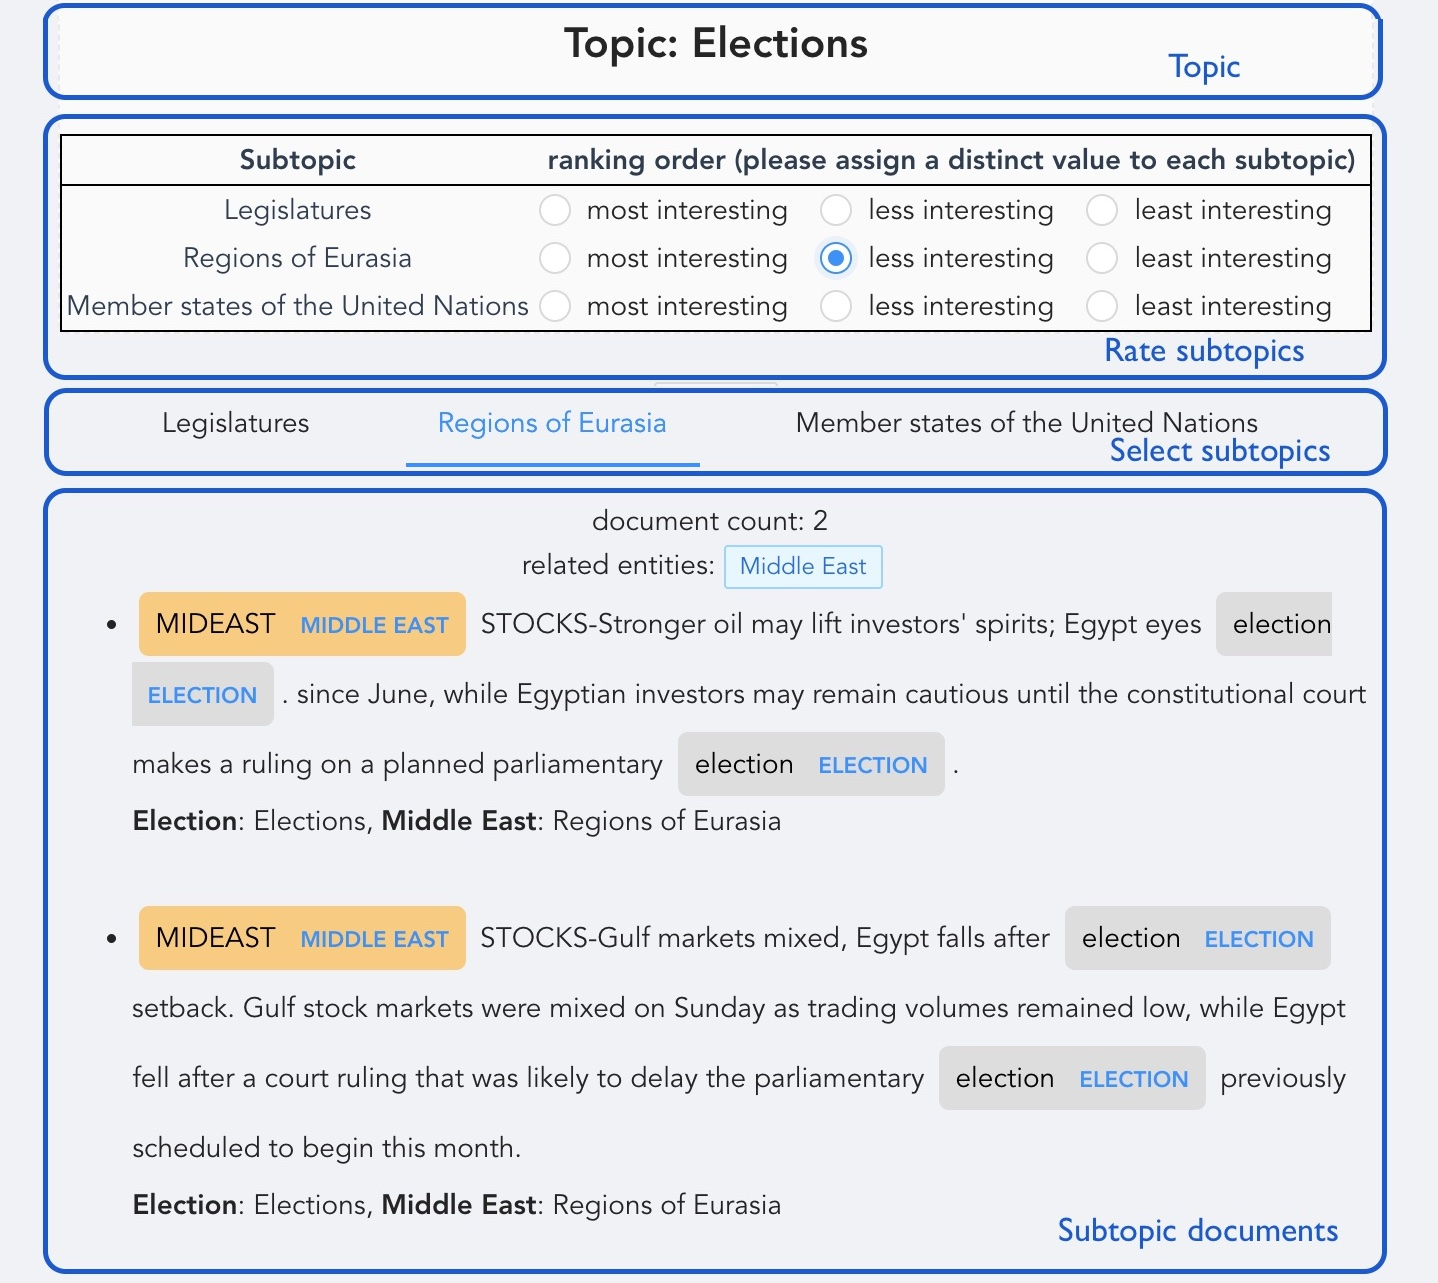}

        \caption{Subtopic survey interface}
        \label{fig:subtopic-survey-interface}
    \end{minipage}
     \begin{minipage}{\linewidth}
        \centering
        \includegraphics[width=\textwidth]{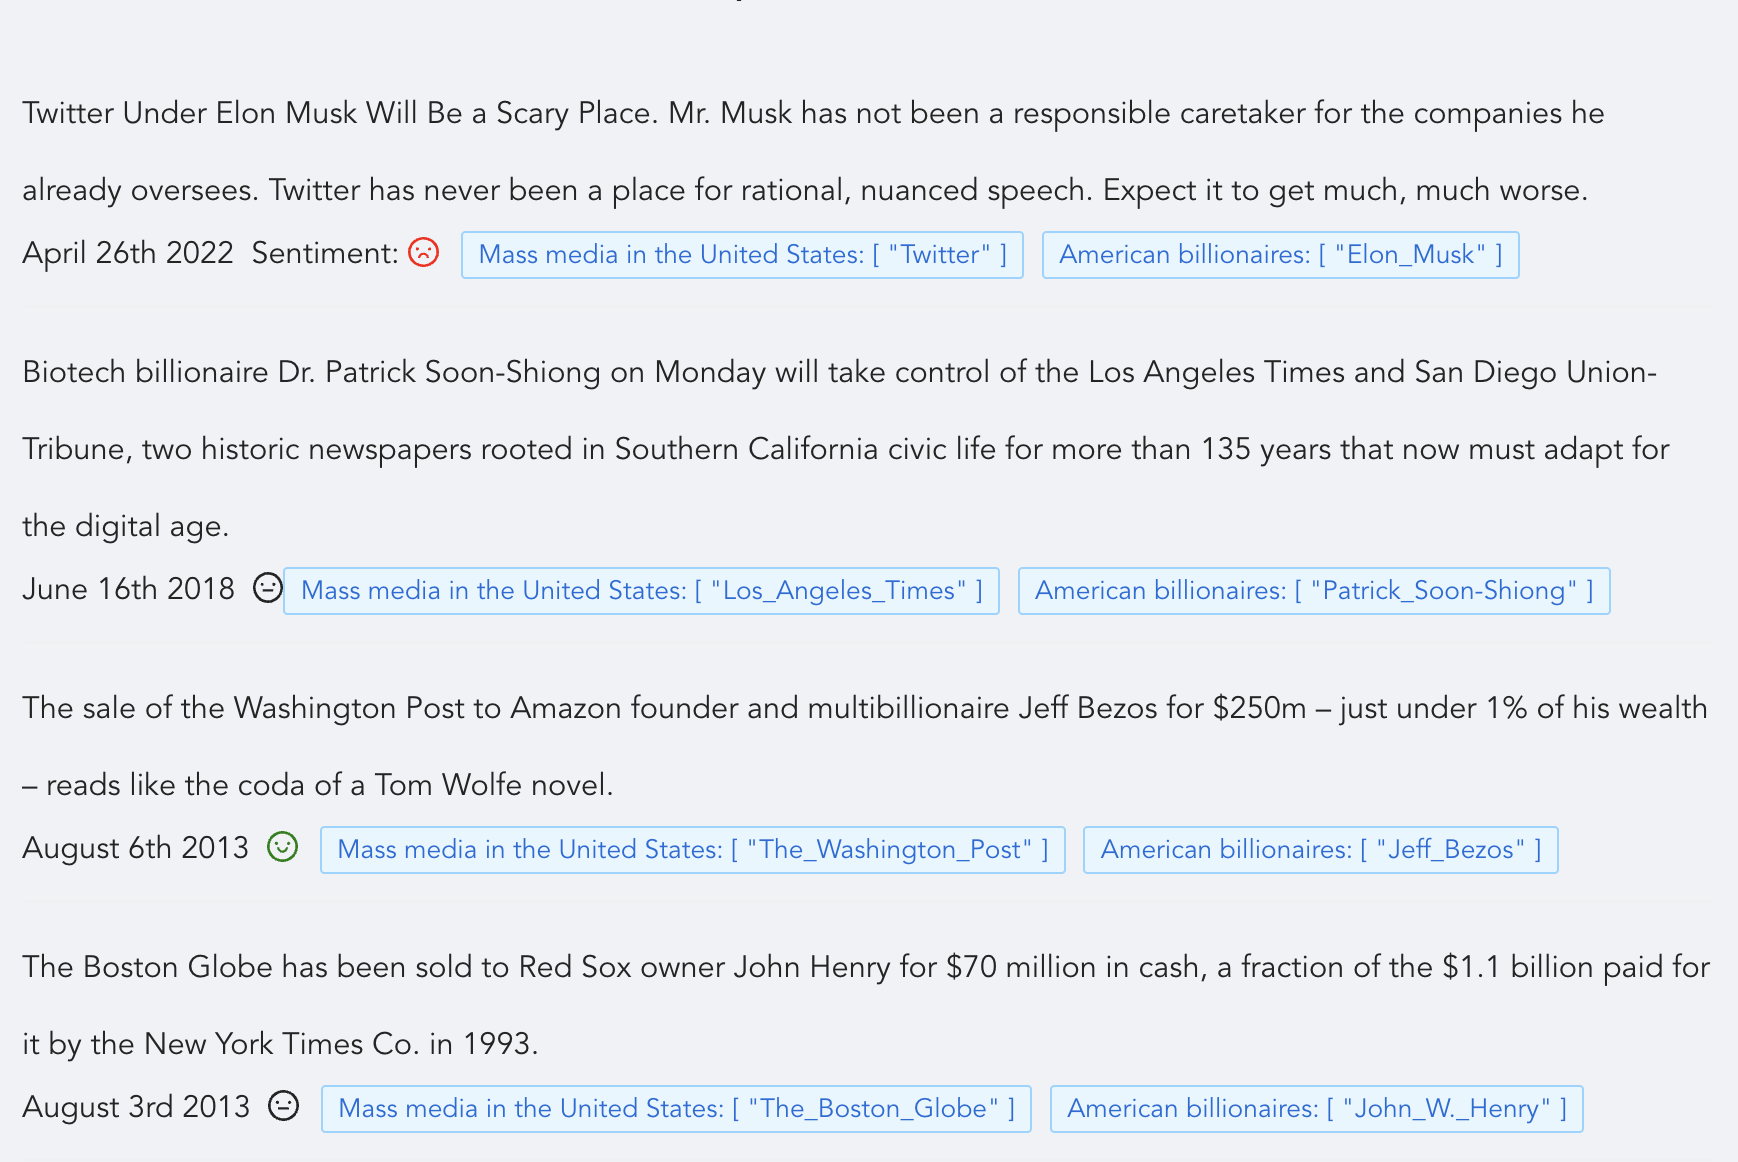}
        \caption{Case study on Media Bias}
        \label{fig:results-with-sentiment}
    \end{minipage}
\end{adjustwidth}
\end{figure}

% \begin{figure}
% \centering
% \begin{adjustwidth}{}{}
    
% \end{adjustwidth}
% \end{figure}
